# Supplementary material for: Precision tests of the AdS/CFT correspondence
Source: arXiv:2611.37641 source file (2026-11-27)
Supplement: Supplementary file 1 [file myappendix.tex]

% !TeX root = ../../thesis.tex
\chapter{More details on Log corrections}\label{ch:myappendix}


%\instructionsappendices

%%%%%%%%%%%%%%%%%%%%%%%%
\addtocontents{toc}{\protect\setcounter{tocdepth}{1}}
%%%%%%%%%%%%%%%%%%%%%%%%


%%%%%%%%%%%%%%%%%%%%%%%%
\section{Euclidean spinors}
\label{App:Euclid-spinors}
%%%%%%%%%%%%%%%%%%%%%%%%


In this appendix we briefly summarize the 4d Euclidean convention for spinors and gamma matrices, see \cite{VanProeyen:1999ni,deWit:2017cle} for details. We use hermitian gamma matrices satisfying
%
\begin{equation}
(\gamma_a)^\dagger=\gamma_a\,,\qquad\{\gamma_a,\gamma_b\}=2\delta_{ab}\,,
\end{equation}
%
and define the 5th gamma matrix $\gamma^5$ as
%
\begin{equation}
\gamma^5=\gamma_1\gamma_2\gamma_3\gamma_4\,.
\end{equation}
%
The charge conjugation matrix $\Omega$ satisfies
%
\begin{equation}
\Omega = -\Omega^\mathrm{T}\,,\qquad \Omega\gamma_a\Omega^{-1} = -(\gamma_a)^\mathrm{T}\,,\label{eq:calC}
\end{equation}
%
and also the unitarity relation $\Omega^\dagger = \Omega^{-1}$.

In 4d Euclidean signature, Majorana spinors are not irreducible and instead we must use symplectic-Majorana spinors. A symplectic-Majorana spinor $\lambda^i$ satisfies the constraint
%
\begin{equation}
\Omega^{-1}(\bar{\lambda}_{i})^{\mathrm{T}} = \varepsilon_{ij}\,\lambda^j\,, \label{eq:sympMaj}
\end{equation}
%
written in terms of the charge conjugation matrix $\Omega$ and the antisymmetric tensor $\varepsilon_{ij}$ with $\varepsilon_{12} = 1$, 
where the bar is defined as $\bar{\lambda}_i := (\lambda^i)^\dagger$ and SU(2) indices $i,j\in\{1,2\}$ are raised and lowered by complex conjugation. The symplectic-Majorana condition \eqref{eq:sympMaj} yields the following useful identities on bilinears of \emph{anti-commuting} symplectic-Majorana spinors:
%
\begin{equation}
\label{eq:sM-bil-aC}
\bigl(\bar{\lambda}_j\,\Gamma^\dagger\,\varphi^i\bigr)^\dagger = \bar{\varphi}_i\,\Gamma\,\lambda^j = -\varepsilon_{ik}\,\varepsilon^{jl}\,\bar{\lambda}_l\,\Omega^{-1}\Gamma^{\mathrm{T}}\Omega\,\varphi^k \, ,
\end{equation}
%
where $\Gamma$ is any combination of gamma matrices. For \emph{commuting} symplectic-Majorana spinors, we have instead
%
\begin{equation}
\label{eq:sM-bil-C}
\bigl(\bar{\lambda}_j\,\Gamma^\dagger\,\varphi^i\bigr)^\dagger = \bar{\varphi}_i\,\Gamma\,\lambda^j = \varepsilon_{ik}\,\varepsilon^{jl}\,\bar{\lambda}_l\,\Omega^{-1}\Gamma^{\mathrm{T}}\Omega\,\varphi^k \, ,
\end{equation}
%
where the additional minus sign comes from $(AB)^\mathrm{T} = -B^\mathrm{T}A^\mathrm{T}$ for two Grassmann-odd matrices $A$ and $B$.


%%%%%%%%%%%%%%%%%%%%%%%%
\section{Trace computations}
\label{App:coeffs}
%%%%%%%%%%%%%%%%%%%%%%%%


In this appendix, we study the quadratic operator $\mathcal{Q}$ and the associated bulk contribution to the fourth SdW coefficient in~\eqref{eq:a4-bulk}. We do so for all massless and massive quantum fluctuations of fields with spin $0\leq s\leq 2$. For $s=0$ and $s=1/2$ we study the fluctuations around a generic Einstein-Maxwell background satisfying the equations of motion \eqref{eom}, while for spin $1\leq s\leq 2$ we turn off the background graviphoton and focus on Einstein backgrounds for simplicity.


%%%%%%%%%%%%%%%%%%%%%%%%
\subsection{Scalar fluctuations}
\label{App:coeffs-scal}
%%%%%%%%%%%%%%%%%%%%%%%%


The Euclidean action for scalar fluctuations to quadratic order reads
%
\begin{equation}
S = \int d^4x \sqrt{g}\,\phi\bigl[-\mathcal{D}^\mu\mathcal{D}_\mu + m^2\bigr]\phi \, ,\label{S:0}
\end{equation}
%
where the covariant derivative is
%
\begin{equation}
\mathcal{D}_\mu\phi = \nabla_\mu\phi - \mathrm{i}\,q\,A_\mu\,\phi \, .
\end{equation}
%
Here, $q$ is the charge of the scalar field with respect to the background graviphoton. The quadratic operator can be read off from the action \eqref{S:0} as
%
\begin{equation}
\mathcal{Q}_{\text{scal}} = \mD^\mu\mD_\mu - m^2 \, . 
\end{equation}
%
The associated quantities for the trace computations are defined in Section~\ref{sec:sugra:local} and are given by
%
\begin{equation}
E = -m^2 \, , \qquad \Omega_{\mu\nu} = -\mathrm{i}\,q\,F_{\mu\nu} \, .\label{Q-component:0}
\end{equation}
%
Substituting \eqref{Q-component:0} into the trace formula \eqref{eq:a4-details:bulk} and then rewriting the result in terms of the 4-derivative quantities as in \eqref{eq:a4-bulk}, we obtain the heat kernel coefficients
%
\begin{equation}
a_E = \frac{1}{360} \, , \quad c = \frac{1}{120} \, , \quad b_1 = \frac{1}{288}\bigl((mL)^2 + 2\bigr)^2 \, , \quad b_2 = \frac{1}{144}\,(q L)^2 \, ,\label{coeffi:0}
\end{equation}
%
where we have also used the background equations of motion \eqref{eom}. The heat kernel coefficients for the massless case can be obtained simply by setting $m^2=-2/L^2$ in \eqref{coeffi:0}.


%%%%%%%%%%%%%%%%%%%%%%%%
\subsection{Spinor fluctuations}
\label{App:coeffs-ferm}
%%%%%%%%%%%%%%%%%%%%%%%%


The Euclidean action for massive symplectic-Majorana spinors is given by \cite{deWit:2017cle}\footnote{The Euclidean Dirac action in a similar form can be derived by generalizing the Wick rotation to spinors~\cite{vanNieuwenhuizen:1996tv}. A proper derivation of the Euclidean spinor action from conformal supergravity was implemented in~\cite{deWit:2017cle}.}
%
\begin{equation}
S = \int d^4x \sqrt{g}\,\bar{\psi}_i\gamma^5\bigr[\delta^i{}_j\,\slashed{\mathcal{D}} - m\,\sigma_3{}^i{}_j\bigr]\psi^j \equiv \int d^4x \sqrt{g}\,\bar{\psi}\,\mathbb{D}\,\psi \, ,
\end{equation}
%
where the covariant derivative is
%
\begin{equation}
\mathcal{D}_\mu\Omega^i = \nabla_\mu\Omega^i - \mathrm{i}\,q\,\sigma_3{}^i{}_j\,A_\mu\Omega^j \, ,
\end{equation}
%
and $\sigma_3$ is the third Pauli matrix. To obtain a Laplace-type differential operator, we square the massive Dirac operator to $\mathcal{Q}_{\text{ferm}} = -\mathbb{D}^2$, see e.g. \cite{Vassilevich:2003xt}, and use
%
\begin{equation}
\log\det\mathbb{D} = \frac12\log\det\mathcal{Q}_\text{ferm} \, .
\end{equation}
%
The resulting second-order operator reads
%
\begin{equation}
\label{eq:Laplace-ferm}
\mathcal{Q}_{\text{ferm}} = \delta^i{}_j\bigg(\mD^\mu\mD_\mu - \frac14\,R - m^2\bigg) \, ,
\end{equation}
%
where the Ricci scalar term arises due to the Lichnerowicz formula based on the identity $\gamma^{ab}\gamma^{cd}R_{abcd}=-2R$. This operator is diagonal in the SU(2) indices. Thus, to obtain the contribution to the heat kernel coefficients from a single symplectic-Majorana spinor, we can work with the above $\mathcal{Q}_{\text{ferm}}$ and divide the final result by four: one factor of two for the SU(2) indices and another factor of two for the symplectic-Majorana condition. From~\eqref{eq:Laplace-ferm} we read off the matrices
%
\begin{equation}
\begin{split}
E =&\; - \frac14\bigl(R + 4m^2\bigr)\delta^i_j - \frac12\mathrm{i}\,q\,F_{ab}\gamma^{ab}\,\sigma_3{}^i{}_j \, , \\
\Omega_{\mu\nu} =&\; \frac14\,R^{ab}{}_{\mu\nu}\gamma_{ab}\,\delta^i_j - \mathrm{i}\,q\,F_{\mu\nu}\,\sigma_3{}^i{}_j \, ,
\end{split}\label{Q-component:1/2}
\end{equation}
%
defined in Section~\ref{sec:sugra:local}. Substituting \eqref{Q-component:1/2} into the trace formula \eqref{eq:a4-details:bulk} and then rewriting the result in terms of the 4-derivative quantities in \eqref{eq:a4-bulk}, we obtain the heat kernel coefficients
%
\begin{equation}
a_E = -\frac{11}{720} \, , \quad c = -\frac{1}{40} \, ,\quad b_1 = \frac{1}{144}(mL)^2\bigl((mL)^2 - 2\bigr) \, , \quad b_2 = -\frac{1}{36}(qL)^2 \, ,\label{coeffi:1/2}
\end{equation}
%
for a single massive spin-1/2 field. The heat kernel coefficients for the massless case can be obtained simply by setting $m=0$ in \eqref{coeffi:1/2}.


%%%%%%%%%%%%%%%%%%%%%%%%
\subsection{Vector fluctuations}
\label{App:coeffs-vec}
%%%%%%%%%%%%%%%%%%%%%%%%


For a massless Abelian spin-1 field, the Euclidean action reads
%
\begin{equation}
S = \int d^4 x \sqrt{g}\,\bigg[-\frac14\,F^{\mu\nu}F_{\mu\nu} - \frac12\,(\nabla^\mu A_\mu)^2\bigg] \, ,
\end{equation}
%
where we include a gauge-fixing term imposing the gauge $\nabla^\mu A_\mu = 0$. To consider the massive case, we introduce a Stückelberg scalar $B$ and consider the action \cite{Ruegg:2003ps}
%
\begin{equation}
\label{eq:spin-1-S}
S = \int d^4 x \sqrt{g}\,\bigg[-\frac14\,F^{\mu\nu}F_{\mu\nu} - \frac12\,\bigl(m\,A_\mu + \nabla_\mu B\bigr)^2 - \frac12\,\bigr(\nabla^\mu A_\mu + m\,B\bigl)^2\bigg] \, .
\end{equation} 
%
Note that the first two terms are invariant under
%
\begin{equation}
\delta A_\mu = \nabla_\mu \lambda \, , \qquad \delta B = - m\,\lambda \, ,
\end{equation}
%
and that the last term is the new gauge-fixing term for this symmetry. To enforce the gauge at the quantum level, we introduce anticommuting scalar ghost and anti-ghost fields with action
%
\begin{equation}
S_{\text{gh}} = \int d^4x \sqrt{g}\,\bar{b} \bigl[-\nabla^\mu\nabla_\mu + m^2\bigr] c \, .
\end{equation}
%
The gauge-fixing term allows us to write the action \eqref{eq:spin-1-S} in terms of a Laplace-type quadratic operator. This operator is diagonal in field space and reads
%
\begin{equation}
\label{eq:Q-vec}
\mathcal{Q}_{\text{vec}} = \begin{pmatrix} g^{\mu\nu}\bigl(\nabla^2 - m^2\bigr) - R^{\mu\nu} \;& 0 \\ 0 \;& \nabla^2 - m^2 \end{pmatrix} \, .
\end{equation}
%
From this we can read off the following matrices defined in Section~\ref{sec:sugra:local},
%
\begin{equation}
E = \begin{pmatrix} -m^2 g^{\mu\nu} - R^{\mu\nu} \;& 0 \\ 0 \;& -m^2 \end{pmatrix} \, , \quad \Omega_{\rho\sigma} = \begin{pmatrix} R^{\mu\nu}{}_{\rho\sigma} \;& 0 \\ 0 \;& 0 \end{pmatrix} \, .
\end{equation}
%
This leads to the following heat kernel coefficients for the physical fields,
%
\begin{equation}
a_E^{\text{ph}} = \frac{13}{72} \, , \qquad c^{\text{ph}} = \frac{1}{8} \, ,\qquad b_1^{\text{ph}} = \frac{1}{288}\bigl(5(mL)^4 - 4(mL)^2 + 12\bigr) \, , \label{coeffi:1-ph}
\end{equation}
%
based on the trace formula \eqref{eq:a4-details:bulk} and the equivalent expression \eqref{eq:a4-bulk} under the background equations of motion \eqref{eom} with a vanishing background graviphoton. The ghost sector contributes minus twice the coefficients for a real scalar field \eqref{coeffi:0}, namely 
%
\begin{equation}
a_E^{\text{gh}} = -\fft{1}{180} \, , \qquad c^{\text{gh}} = -\fft{1}{60} \, ,\qquad b_1^{\text{gh}} = -\fft{1}{144}((mL)^2+2)^2 \, , \label{coeffi:1-gh}
\end{equation}
%
where the factor of two accounts for the pair of ghost and anti-ghost fields and the minus sign arises due to their anticommuting nature. 

Putting the contribution from the physical sector \eqref{coeffi:1-ph} and ghost sector \eqref{coeffi:1-gh} together, we arrive at the following heat kernel coefficients for a massive Abelian vector field
%
\begin{equation}
a_E = \frac{7}{40} \, , \qquad c = \frac{13}{120} \, ,\qquad b_1 = \frac{1}{288}\bigl(3(mL)^4 - 12(mL)^2 + 4\bigr) \, .\label{coeffi:1}
\end{equation}
%
Note that in these trace computations, the Stückelberg field $B$ effectively adds a simple scalar degree of freedom to the coefficients obtained from the vector and ghost fields. This is a manifestation of the fact that the quadratic operator~\eqref{eq:Q-vec} is diagonal in field space. One can check that the heat kernel coefficients for a massless Abelian vector field presented in \cite{David:2021eoq}
%
\begin{equation}
a_E = \frac{31}{180} \, , \qquad c = \frac{1}{10} \, ,\qquad b_1 = 0 \, ,\label{coeffi:1-ml}
\end{equation}
%
are indeed equivalent to the result obtained by subtracting \eqref{coeffi:0} from \eqref{coeffi:1} with $m=0$.


%%%%%%%%%%%%%%%%%%%%%%%%
\subsection{Gravitino fluctuations}
\label{App:coeffs-gravitino}
%%%%%%%%%%%%%%%%%%%%%%%%


The Euclidean action for a massive gravitino field reads
%
\begin{equation}
\label{eq:RS}
S = \int d^4x \sqrt{g}\,\bigg(\bar{\psi}_{\mu i}\,\gamma^5\bigl[\delta^i{}_j\gamma^{\mu\nu\rho}\mathcal{D}_\nu - m\,\sigma_3{}^i{}_j\,\gamma^{\mu\rho}\bigr]\psi_{\rho}{\!}^j + \frac12\mathrm{i}\,F^{\rho\sigma}\,\bar{\psi}_{\mu i}\gamma^5\gamma_\rho\gamma^{\mu\nu}\gamma_\sigma\psi_\nu{\!}^i\bigg) \, ,
\end{equation}
%
where $\mathcal{D}_\mu$ denotes the covariant derivative. In the following we will turn off the background gauge field and focus on the gravitino fluctuation around a general Einstein background. The Rarita-Schwinger action above needs to be modified to include a symplectic-Majorana St\"uckelberg field $\chi^i$ as\footnote{See \cite{Porrati:2008ha} and references therein for how the Stückelberg formalism works for a Rarita-Schwinger field in the Lorentzian signature. Here we generalized it to the Euclidean signature based on \cite{deWit:2017cle}. Note also that we use $\nabla_{\mu}$ and not the more general covariant derivative $\mathcal{D}_\mu$ since we are considering backgrounds with vanishing graviphoton.} 
%
\begin{equation}
\label{eq:RS-S}
S_\chi = \int d^4x \sqrt{g}\,\Bigl(\bar{\psi}_{\mu i} + \frac{1}{m}\,\nabla_\mu\bar{\chi}_i\,\gamma^5\Bigr)\,\gamma^5\bigl[\delta^i{}_j\,\gamma^{\mu\nu\rho}\nabla_\nu - m\,\sigma_3{}^i{}_j\,\gamma^{\mu\rho}\bigr]\Bigl(\psi_\rho{\!}^j + \frac{1}{m}\,\gamma^5\nabla_\rho\chi^j\Bigr) \, .
\end{equation}
%
Implementing the field redefinition
%
\begin{equation}
\label{eq:grav-shift}
\psi_\mu{\!}^i \to \psi_\mu{\!}^i + \frac12\,\sigma_3{}^i{}_j\,\gamma_\mu\gamma^5\chi^j \, ,
\end{equation}
%
the modified action can be written in the form
%
\begin{equation}
\label{eq:start-Stuck}
\begin{split}
S_\chi = S - \int d^4x \sqrt{g}\,&\bigg(\frac32\,\bar{\chi}_i\gamma^5\slashed{\nabla}\chi^i - 3\,m\,\bigl[\sigma_3{}^i{}_j\,\bar{\chi}_i\gamma^5\chi^j + \bar{\psi}_{\mu i}\gamma^\mu\chi^i\bigr] \\
&- \frac{1}{4m}\Bigl[R\,\sigma_3{}^i{}_j\,\bar{\chi}_i\gamma^5\chi^j - 4\,G^{\mu\nu}\bar{\psi}_{\mu i}\gamma_\nu\chi^i + \frac{2}{m}\,G^{\mu\nu}\bar{\chi}_i\gamma^5\gamma_\mu\nabla_\nu\chi^i\Bigr]\bigg) \, ,
\end{split}
\end{equation}
%
where $G_{\mu\nu}$ is the Einstein tensor. After the shift~\eqref{eq:grav-shift}, the action $S$ in~\eqref{eq:RS-S} is invariant under the BRST transformations
%
\begin{equation}
\begin{alignedat}{2}
\delta_B \psi_\mu{\!}^i &= \nabla_\mu c^i - \frac{m}{2}\,\sigma_3{}^i{}_j\,\gamma_\mu c{\,}^j \, ,&\qquad \delta_B \chi^i &= -m\gamma^5 c^i \, , \\
\delta_B b^i &= \mathrm{i}\,\gamma^5\slashed{\nabla} B^i\,,&\qquad \delta_B c^i &= 0 \, , \qquad\qquad \delta_B B^i = 0 \, ,
\end{alignedat}
\end{equation}
%
where $b^i$ and $c^i$ are commuting symplectic-Majorana ghosts and $B^i$ is an anti-commuting symplectic-Majorana Nakanishi-Lautrup field. To consistently fix the gauge, we introduce the BRST-invariant action
%
\begin{equation}
\label{eq:3/2-gf-action}
S_{\text{gf}} = \int d^4x \sqrt{g}\,\Bigl(\mathrm{i}\,\delta_B\bigl[\,\bar{b}_i\,\mathcal{G}^i\,\bigr] + \xi\,\bar{B}_i\gamma^5\slashed{\nabla} B^i\Bigr) \, ,
\end{equation}
%
and choose the gauge-fixing function
%
\begin{equation}
\label{eq:harmonic}
\mathcal{G}^i = \gamma^\mu\psi_\mu{\!}^i \, . 
\end{equation}
%
Lastly, we introduce the massless commuting Kallosh-Nielsen ghost $d^{\,i}$ with action
%
\begin{equation}
S_{\text{KN}} = \frac12\,\mathrm{i}\,\int d^4x \sqrt{g}\,\bar{d}_i \slashed{\nabla} d^{\,i} \, .
\end{equation}
%
Upon choosing $\xi = -\frac12$ in~\eqref{eq:3/2-gf-action}, the complete action $S_{\text{tot}} = S_\chi + S_{\text{gf}} + S_{\text{KN}}$ can be written in Dirac form
%
\begin{equation}
S_{\text{tot}} = \Bigl( \bar{\psi}_{\mu i} \;\; \bar{\chi}_i \;\; \bar{b}_i \;\; \bar{d}_i \Bigr)\,\mathbb{D} \begin{pmatrix} \psi_\nu{}^j \\ \chi^j \\ c^{\,j} \\ d^{\,j} \end{pmatrix} \, ,
\end{equation}
%
where
%
\begin{equation}
\label{eq:D}
\mathbb{D} = \begin{pmatrix} \gamma^5[\delta^i_j\,g^{\mu\nu}\slashed{\nabla} - m\sigma_3{}^i{}_j\gamma^{\mu\nu}] & -M\,\delta^i_j\gamma^\mu & 0 & 0 \\[2mm] -M\,\delta^i_j\gamma^\nu & -\gamma^5[\delta^i_j\slashed{\nabla} - 2m\sigma_3{}^i{}_j] & 0 & 0 \\[1.5mm] 0 & 0 & 2\mathrm{i}[\delta^i_j\slashed{\nabla} - 2m\sigma_3{}^i{}_j] & 0 \\[1.5mm] 0 & 0 & 0 & \mathrm{i}\,\delta^i_j\slashed{\nabla} \end{pmatrix} \, .
\end{equation}
%
To write the expressions above, we introduced 
%
\begin{equation}
M = \sqrt{\frac{\Lambda}{2} + \frac32\,m^2} \, , 
\end{equation} 
%
and used that $G_{\mu\nu} = -\Lambda\,g_{\mu\nu}$ for an Einstein background. We further rescaled the St\"uckelberg fermion $\chi^i$ and all the ghosts to normalize all kinetic terms. \\

Since the operator~\eqref{eq:D} is block diagonal, we first focus on the physical sector in the $2\times 2$ upper left corner. To extract the heat kernel coefficients, we square this operator to bring it to the Laplace form \eqref{eq:Laplace-op} and define $\mathcal{Q}_{\text{gravitino}} = -\mathbb{D}^2$, as in the spin-1/2 case. Contrary to the spin-1 case, this operator is not diagonal in field space due to the cross terms between the gravitino and the St\"uckelberg fermion:
%
\begin{equation}
\mathcal{Q}_{\text{gravitino}} = \begin{pmatrix} \mathcal{Q}_{\psi\psi} & \mathcal{Q}_{\psi\chi} \\[1mm] -\mathcal{Q}_{\psi\chi} & \mathcal{Q}_{\chi\chi} \end{pmatrix} \, .
\end{equation}
%
Explicitly, we have the following matrix elements:
%
\begin{equation}
\begin{split}
\mathcal{Q}_{\psi\psi} =&\; \delta^i_j\,g^{\mu\nu}\slashed{\nabla}^2 - 4m\,\sigma_3{}^i{}_j\,g^{\rho[\mu}\gamma^{\nu]}\nabla_\rho -\delta^i_j(M^2 + 3m^2)g^{\mu\nu} - \delta^i_j(M^2 + 2m^2)\gamma^{\mu\nu} \, , \\[1mm]
\mathcal{Q}_{\chi\chi} =&\; \delta^i_j\slashed{\nabla}^2 - 4\,\delta^i_j(M^2 + m^2) \, , \\[1mm]
\mathcal{Q}_{\psi\chi} =&\; 2M\,\delta^i_j\,\gamma^5\nabla^\mu - 5mM\,\sigma_3{}^i{}_j\,\gamma^5\gamma^\mu \, ,
\end{split}
\end{equation}
%
which leads to the following field space matrix for $E$,
%
\begin{equation}
\begin{split}
E_{\psi\psi} =&\; \frac12\,\delta^i_j\,\bigg(R^{\mu\nu}{}_{ab}\gamma^{ab} - \frac12\,R\,g^{\mu\nu} + 6m^2\,g^{\mu\nu} - 2M^2\,\gamma^{\mu\nu}\bigg) \, , \\[1mm]
E_{\chi\chi} =&\; -\frac14\,\delta^i_j\,\bigl(R + 16m^2\bigr) \, , \\[1mm]
E_{\psi\chi} =&\; -E_{\chi\psi} = -2mM\,\sigma_3{}^i{}_j\,\gamma^5\gamma^\mu \, ,
\end{split}
\end{equation}
%
and for $\Omega_{\rho\sigma}$,
%
\begin{align}
(\Omega_{\rho\sigma})_{\psi\psi} =&\; \delta^i_j\,\bigg(R^{\mu\nu}{}_{\rho\sigma} + \frac14\,g^{\mu\nu}R_{\rho\sigma ab}\gamma^{ab} + 2m^2\Bigl[\gamma^\mu\gamma_{[\rho}g_{\sigma]}{}^\nu + g^\mu{}_{[\rho}\gamma_{\sigma]}\gamma^\nu - \Bigl(4 + \frac{M^2}{m^2}\Bigr)g^{\mu}{}_{[\rho}g_{\sigma]}{}^\nu\Bigr]\bigg) \, , \nonumber \\[1mm]
(\Omega_{\rho\sigma})_{\chi\chi} =&\; \frac14\,\delta^i_j\,R_{\rho\sigma a b}\gamma^{ab} \, , \\[1mm]
(\Omega_{\rho\sigma})_{\psi\chi} =&\; -(\Omega_{\rho\sigma})_{\chi\psi} = 2mM\,\sigma_3{}^i{}_j\,\gamma^5 g^\mu{}_{[\rho}\gamma_{\sigma]} \, . \nonumber
\end{align}
%
With this at hand, we obtain the heat kernel coefficients for the physical sector
%
\begin{equation}
a_E^{\text{ph}} = \frac{109}{36} \, , \qquad c^{\text{ph}} = \frac{25}{6} \, ,\qquad b_1^{\text{ph}} = \frac{1}{18}\bigl(17(mL)^4 - 16(mL)^2 + 11\bigr) \, ,\label{coeffi:3/2:ph}
\end{equation}
%
based on the trace formula~\eqref{eq:a4-details:bulk} and the equivalent expression~\eqref{eq:a4-bulk} obtained using the background equations of motion \eqref{eom}. The ghost sector does not present additional complications and the corresponding heat kernel coefficients can be evaluated using the $2\times 2$ lower right corner of the operator \eqref{eq:D}. The result is given by
%
\begin{equation}
a_E^{\text{gh}} = \frac{11}{60} \, , \qquad c^{\text{gh}} = \frac{3}{10} \, ,\qquad b_1^{\text{gh}} = -\fft49(mL)^2(2(mL)^2-1) \, ,\label{coeffi:3/2:gh}
\end{equation}
%
where we have taken into account the overall minus sign due to the opposite spin statistics of the ghosts fields (commuting) with respect to the physical fields (anti-commuting). 

Summing the contribution from the physical sector \eqref{coeffi:1-ph} and the ghost sector \eqref{coeffi:1-gh} and dividing the final result by four as in the spin-1/2 case, we obtain the heat kernel coefficients
%
\begin{equation}
a_E = \frac{289}{360} \, , \qquad c = \frac{67}{60} \, ,\qquad b_1 = \frac{1}{72}\bigl((mL)^4 - 8(mL)^2 + 11\bigr) \, ,\label{coeffi:3/2}
\end{equation}
%
for a single massive spin-3/2 field. The heat kernel coefficients for a massless spin-3/2 fluctuation can be computed in the same way but without the contribution from the spin-1/2 St\"uckelberg field. The final result is given by
%
\begin{equation}
a_E = \frac{589}{720} \, , \qquad c = \frac{137}{120} \, ,\qquad b_1 = 0 \, .\label{coeffi:3/2-ml}
\end{equation}


%%%%%%%%%%%%%%%%%%%%%%%%
\subsection{Graviton fluctuations}
\label{App:coeffs-graviton}
%%%%%%%%%%%%%%%%%%%%%%%%


The Euclidean action for a massive spin-2 fluctuation $h_{\mu\nu}$ is given by adding the Pauli-Fierz mass term to the massless action and reads
%
\begin{equation}
\begin{split}
S = \int d^4x \sqrt{g}\,\Bigl[&h^{\mu\nu}\nabla^\rho \nabla_\rho h_{\mu\nu}-h\nabla^\mu \nabla_\mu h+2h \nabla_\mu \nabla_\nu h^{\mu\nu}+2\nabla_\nu h^{\mu\nu}\nabla_\rho h_\mu{}^\rho\\
&+2h^{\mu\nu}h^{\rho\sigma}R_{\mu\rho\nu\sigma}+2h_{\mu\nu}h^{\mu\rho}R^\nu{}_\rho-2h^{\mu\nu}hR_{\mu\nu}-h^{\mu\nu}h_{\mu\nu}R+\frac12h^2R\\
&+\Lambda(2h_{\mu\nu}h^{\mu\nu}-h^2)-m^2(h_{\mu\nu}h^{\mu\nu}-h^2)\Bigr] \, ,
\end{split}
\end{equation}
%
where all curvature tensors are those of the background metric $g_{\mu\nu}$ and $h = h^\mu{}_\mu$. As in the previous cases for spin-1 and spin-3/2 fields, the Pauli-Fierz mass term breaks the local gauge invariance. We can restore the symmetry by introducing two Stückelberg fields, namely a scalar $\phi$ and a vector $B_\mu$, and replace the metric fluctuation by
%
\begin{equation}
h_{\mu\nu} \to h_{\mu\nu}-\frac12\,g_{\mu\nu}\phi+\frac1m \nabla_\mu\Bigl(B_\nu-\frac{1}{2m}\nabla_\nu\phi\Bigr)+\frac1m \nabla_\nu\Bigl(B_\mu-\frac{1}{2m}\nabla_\mu\phi\Bigr) \, ,
\end{equation}
%
see for example \cite{Porrati:2008ha} and references therein. The resulting action now enjoys the gauge symmetry
%
\begin{equation}
\delta h_{\mu\nu} = \nabla_\mu\xi_\nu + \nabla_\nu\xi_\mu + \lambda\,m\,g_{\mu\nu} \, , \quad \delta B_\mu = \nabla_\mu\lambda - m\,\xi_\mu \, , \quad \delta \phi = 2m\,\lambda \, ,
\end{equation}
%
for which we add appropriate gauge-fixing terms, 
%
\begin{equation}
\begin{split}
S_{1} =&\; -2\int d^4x\sqrt{g}\,\Bigl(\nabla_\nu h^{\mu\nu} - \frac12\nabla^\mu h + m B^\mu\Bigr)^2 \, , \\
S_{2} =&\; -2\int d^4x\sqrt{g}\,\Bigl(\nabla_\mu B^\mu + \frac{m}{2}(h - 3\phi)\Bigr)^2 \, .
\end{split}
\end{equation}
%
Then, tedious but straightforward manipulations show that the resulting gauge-fixed action $S_\text{gf} = S + S_1 + S_2$ can be written as
%
\begin{equation}
\label{eq:spin-2-m-gf}
\begin{split}
S_{\text{gf}} = \int d^4x \sqrt{g}\,\Bigl\{&h^{\mu\nu}\Bigl[G_{\mu\nu\rho\sigma}(\nabla^2 - m^2) + 2R_{\mu\rho\nu\sigma} - 2g_{\mu\rho}R_{\nu\sigma} + 2\Lambda G_{\mu\nu\rho\sigma}\Bigr]h^{\rho\sigma}\\
&+ B^\mu\bigl[g_{\mu\nu}(\nabla^2 - m^2 + \Lambda)\bigr]B^\nu + \phi\bigl[\nabla^2 - m^2 - 3\Lambda M^{-2}\bigr]\phi\\
&+ 2\Lambda M^{-1} h\,\phi -2\sqrt2\Lambda (mM)^{-1}B^\mu\nabla_\mu\phi\Bigr\} \, ,
\end{split}
\end{equation}
%
where
\begin{equation}
G_{\mu\nu\rho\sigma} = \frac12\bigl(g_{\mu\rho}g_{\nu\sigma} + g_{\mu\sigma}g_{\nu\rho} - g_{\mu\nu}g_{\rho\sigma}\bigr) \, , \qquad M = \sqrt{\frac32 - \frac{\Lambda}{m^2}} \, ,
\end{equation}
%
and we have rescaled the fields to ensure canonically normalized kinetic terms. In deriving~\eqref{eq:spin-2-m-gf}, we made extensive use of the background equations of motion \eqref{eom} with a vanishing graviphoton. We can now read off the Laplace-type operator \eqref{eq:Laplace-op} from \eqref{eq:spin-2-m-gf},
%
\begin{equation}
\mathcal{Q}_{\text{graviton}} = \begin{pmatrix} \mathcal{Q}_{hh} \,& 0 \,& \mathcal{Q}_{h\phi} \\[1mm] 0 \,& \mathcal{Q}_{BB} \,& \mathcal{Q}_{B\phi} \\[1mm] \mathcal{Q}_{h\phi} \,& -\mathcal{Q}_{B\phi} \,& \mathcal{Q}_{\phi\phi} \end{pmatrix} \, .
\end{equation}
%
Just as in the spin-3/2 case we note that this is not diagonal in field space, indicating non-trivial interactions between the graviton fluctuations and the Stückelberg fields. Extracting the matrices $E$ and $\Omega_{\rho\sigma}$ defined in Section \ref{sec:sugra:local} from the operator $\mQ_\text{graviton}$ is straighforward, and we obtain the following heat kernel coefficients from the physical sector:
%
\begin{equation}
a_E^{\text{ph}} = \frac{89}{24} \, , \qquad c^{\text{ph}} = \frac{113}{24} \, ,\qquad b_1^{\text{ph}} = \frac{1}{288}\Bigl(15(mL)^4 + 48(mL)^2 + 256\Bigr) \, ,\label{coeffi:2:ph}
\end{equation}
%
based on the trace formula \eqref{eq:a4-details:bulk} and the equivalent expression \eqref{eq:a4-bulk}. The gauge-fixing introduces a pair of vector ghosts and a pair of scalar ghosts whose Euclidean action reads
%
\begin{equation}
\begin{split}
S_{\text{gh}} = \int d^4x \sqrt{g}\,\Bigl(b_\mu\bigl[g^{\mu\nu}(\nabla^2 - m^2) + R^{\mu\nu}\bigr]c_\nu + b\bigl[\nabla^2 - m^2\bigr]c\Bigr) \, .
\end{split}
\end{equation}
%
Their contribution to the heat kernel coefficients can be obtained from the spin-1 and spin-0 cases treated above. The result is given by
%
\begin{equation}
a_E^{\text{gh}} = -\frac{13}{36} \, , \qquad c^{\text{gh}} = -\fft14 \, ,\qquad b_1^{\text{gh}} = \frac{1}{144}\Bigl(-5(mL)^4 -44(mL)^2 -108\Bigr) \, ,\label{coeffi:2:gh}
\end{equation}
%
where we have included an overall minus sign due to the anticommuting nature of the ghosts.

Putting the physical sector \eqref{coeffi:2:ph} and the ghost sector \eqref{coeffi:2:gh} together, we arrive at our final result
%
\begin{equation}
a_E = \frac{241}{72} \, , \qquad c = \frac{107}{24} \, ,\qquad b_1 = \frac{5}{288}\bigl((mL)^4 - 8(mL)^2 + 8\bigr) \, ,
\end{equation}
%
for the massive spin-2 fluctuations around a generic Einstein background. The heat kernel coefficients for a massless fluctuation can be computed in the same way but without the contribution from St\"uckelberg fields and the corresponding scalar ghosts. The final result is given by
%
\begin{equation}
a_E = \frac{571}{180} \, , \qquad c = \frac{87}{20} \, ,\qquad b_1 = 0 \, .\label{coeffi:2-ml}
\end{equation}


%%%%%%%%%%%%%%%%%%%%%%%%
\section{Rarita-Schwinger zero modes on EAdS$_4$} 
\label{App:RS-non-local}
%%%%%%%%%%%%%%%%%%%%%%%%


In Section~\ref{sec:sugra:non-local-AdS4}, we discussed how
%
\begin{equation}
\Psi^s_{\mu\ell m}(\lambda) = \mathcal{N}^s_\ell\Bigl(\nabla_\mu + \frac{s}{2L}\,\gamma_\mu\Bigr)\Omega^s_{\ell m} \, ,
\end{equation}
%
is a zero mode of the Rarita-Schwinger operator. Here, $\Omega^s_{\ell m}$ is an eigenspinor of the Dirac operator on EAdS$_4$,
%
\begin{equation}
\slashed{\nabla}\Omega^s_{\ell m} = \frac{\mathrm{i}s}{L}\,\lambda\,\Omega^s_{\ell m} \, .
\end{equation}
%
We note that using the above, we have
%
\begin{equation}
\gamma^\mu\Psi_{\mu\ell m}^s(\lambda) = \frac{s}{L}(2 + \mathrm{i}\lambda)\,\mathcal{N}_\ell^s\,\Omega_{\ell m}^s \, .
\end{equation}
%
Since the path integral over spin-3/2 fluctuations includes a delta function enforcing the harmonic gauge as in~\eqref{eq:harmonic}, we should consider the discrete value
%
\begin{equation}
\label{eq:lambda-fix}
\lambda = 2\mathrm{i} \, .
\end{equation}
%
Indeed, the differential operator relevant for non-zero modes is the Laplace-type operator obtained from~\eqref{eq:RS-op} after introducing the proper gauge-fixing term and the corresponding ghost fields, see Appendix~\ref{App:coeffs-gravitino}. To study the zero modes of that operator, we must impose~\eqref{eq:lambda-fix}.\\

For $\lambda \in \mathrm{i}\mathbb{R}$, the Dirac eigenmodes $\Omega^s_{\ell m}$ are not square-integrable on EAdS$_4$~\cite{Camporesi:1995fb}. Using the defining equation~\eqref{eq:eigenspinors}, we can express the norm of the RS zero-modes in terms of the norm of Dirac eigenmodes as follows:
%
\begin{equation}
\label{eq:Psi-sq}
\langle\Psi^s_{\mu\ell m},\Psi^{\mu s}_{\ell m}\rangle = |\mathcal{N}^s_\ell|^2\Bigl[-\frac{2}{L^2}\langle\Omega^{s}_{\ell m},\Omega^{s}_{\ell m}\rangle + \int d^4x\sqrt{g}\,\nabla^\mu\bigl[(\Omega^{s}_{\ell m})^\dagger \nabla_\mu \Omega^{s}_{\ell m}\bigr]\Bigr]_{\lambda = 2\mathrm{i}} \, .
\end{equation}
%
Note the appearance of a total derivative term, which can potentially renormalize the divergences that arise since the first term is non-normalizable. For explicit computations, we use a coordinate system in which the metric on EAdS$_4$ reads
%
\begin{equation}
\label{eq:metric-eta}
ds^2 = L^2(d\eta^2 + \sinh^2\eta\,d\Omega_3^2) \, ,
\end{equation}
%
where $d\Omega_3^2$ is the line element on $S^3$. In this coordinate system, the unit normal to the $S^3$ boundary is $n^\mu = (L^{-1},0,0,0)$ and the spin-connection has non-vanishing components only along the 3-sphere directions. This reduces the boundary term to
%
\begin{equation}
\int d^4x\sqrt{g}\,\nabla^\mu\bigl[(\Omega^{s}_{\ell m})^\dagger \nabla_\mu \Omega^{s}_{\ell m}\bigr]_{\lambda = 2\mathrm{i}} = \sinh^3y \int_{S^3}(\Omega^{s}_{\ell m})^\dagger \partial_\eta \Omega^{s}_{\ell m}\big\vert_{\eta = y, \lambda = 2\mathrm{i}} \, ,
\end{equation}
%
where we put the boundary at $\eta = y$ with $y$ being large.

The Dirac eigenmodes on EAdS$_4$ are given by~\cite{Camporesi:1995fb}
%
\begin{equation}
\Omega^s_{\ell m} = C_\ell(\lambda)\begin{pmatrix} \phi_{\lambda \ell}(\eta)\,\chi_{\ell m}(\theta) \\ \mathrm{i}\,s\,\psi_{\lambda \ell}(\eta)\,\chi_{\ell m}(\theta)\end{pmatrix} \, ,
\end{equation}
%
where $\chi_{\ell m}(\theta)$ are eigenspinors of the Dirac operator on $S^3$ (whose coordinates we generically denote as $\theta$), $\phi$ and $\psi$ are radial functions expressed in terms of the hypergeometric function ${}_2F_1$, and $C_\ell(\lambda)$ is a normalization constant. For the continuous case $\lambda\in\mathbb{R}$ the normalization can be found in~\cite{Camporesi:1995fb}, but since we want to consider the discrete mode with $\lambda$ fixed and imaginary, this normalization cannot be obtained from requiring that the modes $\Omega^s_{\ell m}$ provide an orthonormal basis. To proceed we note that the radial functions satisfy the differential equations
%
\begin{equation}
\label{eq:diff-eq}
\begin{split}
\partial_\eta\phi_{\lambda\ell} =&\; \frac12\Bigl[\ell \coth\tfrac{\eta}{2} + (\ell+1)\tanh\tfrac{\eta}{2}\Bigr]\phi_{\lambda\ell} - \Bigl[\frac{\lambda^2 + (\ell + 2)^2}{\ell + 2}\Bigr]\phi_{\lambda(\ell+1)} \, , \\[1mm]
\partial_\eta\psi_{\lambda\ell} =&\; \frac12\Bigl[(2\ell + 1)\coth\eta + \sinh^{-1}\eta\Bigr]\psi_{\lambda\ell} - \Bigl[\frac{\lambda^2 + (\ell+2)^2}{\ell + 2}\Bigr]\psi_{\lambda(\ell+1)} \, .
\end{split}
\end{equation}
%
Using this, both the bulk and boundary terms in~\eqref{eq:Psi-sq} can be computed. In terms of 
\begin{equation}
\lVert\chi_{\ell m}\rVert_{S^3} = \int_{S^3}\chi^\dagger_{\ell m}\chi_{\ell m} \, ,
\end{equation}
and $s_y = \sinh y$, the result is
%
\begin{equation}
\begin{split}
\frac{2}{L^2}\langle\Omega^{s}_{0 m},\Omega^{s}_{0 m}\rangle_{\lambda = 2\mathrm{i}} =&\; L^2|C_0(2\mathrm{i})|^2\Bigl(\frac{e^{4y}}{32} - \frac{e^{2y}}{8} + \frac{3}{16} + \mathcal{O}(e^{-2y})\Bigr)\,\lVert\chi_{0 m}\rVert_{S^3}  \, , \\[1mm]
s_y^3 \int_{S^3}(\Omega^{s}_{0 m})^\dagger \partial_\eta \Omega^{s}_{0 m}\big\vert_{\eta = y,\lambda = 2\mathrm{i}} =&\; L^2|C_0(2\mathrm{i})|^2\Bigl(\frac{e^{4y}}{32} - \frac{e^{2y}}{8} + \frac{3}{16} + \mathcal{O}(e^{-2y})\Bigr)\,\lVert\chi_{0 m}\rVert_{S^3}  \, ,
\end{split}
\end{equation}
%
for $\ell = 0$, and
\begin{equation}
\begin{split}
\frac{2}{L^2}\langle\Omega^{s}_{1 m},\Omega^{s}_{1 m}\rangle_{\lambda = 2\mathrm{i}} =&\; L^2|C_1(2\mathrm{i})|^2\Bigl(\frac{e^{4y}}{128} - \frac{25e^{2y}}{288} + \frac{475}{576} + \mathcal{O}(e^{-y})\Bigr)\,\lVert\chi_{1 m}\rVert_{S^3}  \, , \\[1mm]
s_y^3 \int_{S^3}(\Omega^{s}_{1 m})^\dagger \partial_\eta \Omega^{s}_{1 m}\big\vert_{\eta = y,\lambda = 2\mathrm{i}} =&\; L^2|C_1(2\mathrm{i})|^2\Bigl(\frac{e^{4y}}{128} - \frac{e^{2y}}{288} + \frac{41}{192} + \mathcal{O}(e^{-y})\Bigr)\,\lVert\chi_{1 m}\rVert_{S^3}  \, ,
\end{split}
\end{equation}
%
for $\ell = 1$. Results for higher values of $\ell$ can be obtained straightforwardly and follow the same pattern. Namely, we observe a perfect cancellation between bulk and boundary terms when $\ell=0$, while the modes with higher values of $\ell$ only see their leading divergences cancel. Thus, in the large $y$ limit,
%
\begin{equation}
\begin{split}
L^{-2}\langle\Psi^s_{\mu 0 m},\Psi^{\mu s}_{0 m}\rangle =&\; 0 \, , \\
L^{-2}\langle\Psi^s_{\mu \ell m},\Psi^{\mu s}_{\ell m}\rangle =&\; |\mathcal{N}_\ell^s C_\ell(2\mathrm{i})|^2\,\Bigl[h_1(\ell)\,e^{2y} + h_2(\ell)\Bigr]\lVert\chi_{\ell m}\rVert_{S^3} \quad \text{for} \quad \ell >0 \, ,
\end{split}
\end{equation}
%
for some $h_1$ and $h_2$ whose first few values are presented in Table~\ref{tab:RS-ZM}.
%
\begin{table}[h]
	\centering
	\renewcommand*{\arraystretch}{1.5}
	\begin{tabular}{|c||c|c|c|c|c|c|c|c|c|c|c|}
		\hline
		$\ell$ & 0 & 1 & 2 & 3 & 4 & 5 & 6 & 7 & 8 & 9 & 10 \\
		\hline
		$h_1(\ell)$ & 0 & $\frac1{12}$ & $\frac{3}{40}$ & $\frac{3}{50}$ & $\frac{1}{21}$ & $\frac{15}{392}$ & $\frac{1}{32}$ & $\frac{7}{270}$ & $\frac{6}{275}$ & $\frac{9}{484}$ & $\frac{5}{312}$ \\
		\hline
		$h_2(\ell)$ & 0 & $-\frac{11}{18}$ & $-\frac{23}{20}$ & $-\frac{39}{25}$ & $-\frac{118}{63}$ & $-\frac{415}{196}$ & $-\frac{37}{16}$ & $-\frac{1001}{405}$ & $-\frac{716}{275}$ & $-\frac{657}{242}$ & $-\frac{1315}{468}$ \\
		\hline
	\end{tabular}
	\caption{The leading and subleading divergences in the norm of the Rarita-Schwinger zero mode on EAdS$_4$ as a function of the mode number $\ell \geq 0$.\label{tab:RS-ZM}}
\end{table}
%
This shows that the RS zero mode has vanishing norm for $\ell = 0$, but is not square-integrable for $\ell > 0$. As such, it cannot contribute to the non-local contribution $C_\text{non-local}$.


%%%%%%%%%%%%%%%%%%%%%%%%
\section{Heat kernel coefficients for KK supergravities}
\label{App:KK}
%%%%%%%%%%%%%%%%%%%%%%%%


In this appendix we compute the contributions $(a_E,c,b_1)$ to the bulk SdW coefficient in \eqref{eq:a4-bulk} for the KK supergravity compactifications discussed in Section \ref{sec:KK}. As explained at the beginning of this section, we will do all computations for minimally coupled fields and use \eqref{eq:hk-non-min} to reinstate the effect of supersymmetric non-minimal couplings when necessary.


%%%%%%%%%%%%%%%%%%%%%%%%
\subsection{KK supergravity on $S^7$}
\label{App:KK:S7}
%%%%%%%%%%%%%%%%%%%%%%%%


The Weyl dimension formula for the SO(8) representation with Dynkin label $(\lambda_1,\lambda_2,\lambda_3,\lambda_4)$ reads\footnote{We follow the conventions summarized in Appendix A of \cite{Bobev:2021wir}.}
%
\begin{equation} \small 
\begin{split}
&\dim(\lambda_1,\lambda_2,\lambda_3,\lambda_4)\\
&=\fft{1}{4320}(1+\lambda_1)(1+\lambda_2)(1+\lambda_3)(1+\lambda_4)(2+\lambda_1+\lambda_2)(2+\lambda_2+\lambda_3)(2+\lambda_2+\lambda_4)\\
&\quad\times(3+\lambda_1+\lambda_2+\lambda_3)(3+\lambda_1+\lambda_2+\lambda_4)(3+\lambda_2+\lambda_3+\lambda_4)\\
&\quad\times(4+\lambda_1+\lambda_2+\lambda_3+\lambda_4)(5+\lambda_1+2\lambda_2+\lambda_3+\lambda_4)\qquad\qquad\qquad\qquad (\lambda_i\geq0) \, ,
\end{split}\label{Weyl:dim:so(8)}
\end{equation}
%
and $\dim(\lambda_1,\lambda_2,\lambda_3,\lambda_4)\equiv0$ if any of the $\lambda_i$'s are negative. We now combine this formula with the data provided in Tables \ref{tab:coeffs}, \ref{tab:conf-m}, \ref{tab:S7}, and \ref{tab:S7-m} to evaluate the heat kernel coefficients for the KK supergravity theory arising from compactification of 11d supergravity on $S^7$.

The $a_E$ coefficient can be computed by adding the contributions from all KK modes of spin $0 \leq s \leq 2$ in the given SO(8) representation. At fixed KK level $k$, we find
%
\begin{align}
\label{S7:a:bulk}
a_E(k) =&\; \fft{1}{360}\Bigl(\text{dim}(k+2,0,0,0)+\text{dim}(k-2,2,0,0)+\text{dim}(k-2,0,0,0) \nonumber \\
&\qquad\;\; +\text{dim}(k,0,2,0)+\text{dim}(k-2,0,0,2)\Bigr) \nonumber \\
+\fft{11}{720}&\Bigl(\text{dim}(k+1,0,1,0)+\text{dim}(k-1,1,1,0) +\text{dim}(k-2,1,0,1)+\text{dim}(k-2,0,0,1)\Bigr) \nonumber \\[1mm]
&+\Bigl[\fft{31}{180}+\fft{1}{360}\Theta(k-1)\Bigr]\Bigl(\text{dim}(k,1,0,0)+\text{dim}(k-1,0,1,1)+\text{dim}(k-2,1,0,0)\Bigr) \nonumber\\[1mm]
&-\Bigl[\fft{589}{720}-\fft{11}{720}\Theta(k-1)\Bigr]\Bigl(\text{dim}(k,0,0,1)+\text{dim}(k-1,0,1,0)\Bigr) \nonumber \\[1mm]
&+\Bigl[\fft{571}{180}+\Bigl(\fft{31}{180}+\fft{1}{360}\Bigr)\Theta(k-1)\Bigr]\text{dim}(k,0,0,0) \, ,
\end{align}
%
where $\Theta(x \geq 0) = 1$ and $\Theta(x < 0) = 0$. This step function takes into account the fact that the contributions from St\"uckelberg fields are present only for massive fields with $k\geq1$. Using~\eqref{Weyl:dim:so(8)}, the total heat kernel coefficient $a_E^{\text{tot}} = \sum_{k\geq0} a_E(k)$ is given by
\begin{equation}
a_E^{\text{tot}} = \fft{1}{144}\sum_{k=0}^\infty(k+1)(k+2)(k+3)^2(k+4)(k+5) \, .
\end{equation}

The heat kernel coefficient $c$ is computed in a similar manner. Here, we find a perfect cancellation at each KK level:
%
\begin{align}
\label{S7:c:bulk}
c(k) =&\; \fft{1}{120}\Bigl(\text{dim}(k+2,0,0,0)+\text{dim}(k-2,2,0,0)+\text{dim}(k-2,0,0,0) \nonumber\\
&\qquad\;\;+\text{dim}(k,0,2,0)+\text{dim}(k-2,0,0,2)\Bigr) \nonumber\\
+\fft{1}{40}&\Bigl(\text{dim}(k+1,0,1,0)+\text{dim}(k-1,1,1,0)+\text{dim}(k-2,1,0,1)+\text{dim}(k-2,0,0,1)\Bigr) \nonumber\\[1mm]
&+\Bigl[\fft{1}{10}+\fft{1}{120}\Theta(k-1)\Bigr]\Bigl(\text{dim}(k,1,0,0)+\text{dim}(k-1,0,1,1)+\text{dim}(k-2,1,0,0)\Bigr) \nonumber\\[1mm]
&-\Bigl[\fft{137}{120}-\fft{1}{40}\Theta(k-1)\Bigr]\Bigl(\text{dim}(k,0,0,1)+\text{dim}(k-1,0,1,0)\Bigr) \nonumber\\[1mm]
&+\Bigl[\fft{87}{20}+\Bigl(\fft{1}{10}+\fft{1}{120}\Bigr)\Theta(k-1)\Bigr]\text{dim}(k,0,0,0)\\[1mm]
=&\; 0 \, . \nonumber
\end{align}
%
We therefore conclude that $c^{\text{tot}} = \sum_k c(k)$ vanishes after summing over the KK tower.

For the $b_1$ coefficient, we note that since the lowest-lying KK modes with $k=0$ are massless, Table~\ref{tab:coeffs} implies that $b_1(0)=0$. For the contribution from higher KK modes with $k\geq 1$, we use the dictionary between mass and conformal dimension in Table~\ref{tab:conf-m} and obtain
%
\begin{align}
\label{S7:b:bulk}
b_1(k) =&\; s_0\Big(\sqrt{(\fft{k}{2}+1)(\fft{k}{2}-2)}\Big)\text{dim}(k+2,0,0,0)+s_0\Big(\sqrt{(\fft{k}{2}+2)(\fft{k}{2}-1)}\Big)\text{dim}(k,0,2,0)\nonumber\\
&+s_0\Big(\sqrt{(\fft{k}{2}+3)\fft{k}{2}}\Big)\text{dim}(k-2,2,0,0)+s_0\Big(\sqrt{(\fft{k}{2}+4)(\fft{k}{2}+1)}\Big)\text{dim}(k-2,0,0,2)\nonumber\\
&+s_0\Big(\sqrt{(\fft{k}{2}+5)(\fft{k}{2}+2)}\Big)\text{dim}(k-2,0,0,0)\nonumber\\
&+s_{\fft12}\Big(\fft{k+3}{2}-\fft32\Big)\text{dim}(k+1,0,1,0)+s_{\fft12}\Big(\fft{k+5}{2}-\fft32\Big)\text{dim}(k-1,1,1,0)\nonumber\\
&+s_{\fft12}\Big(\fft{k+7}{2}-\fft32\Big)\text{dim}(k-2,1,0,1)+s_{\fft12}\Big(\fft{k+9}{2}-\fft32\Big)\text{dim}(k-2,0,0,1)\nonumber\\
&+s_1\Big(\sqrt{(\fft{k}{2}+1)\fft{k}{2}}\Big)\text{dim}(k,1,0,0)+s_1\Big(\sqrt{(\fft{k}{2}+2)(\fft{k}{2}+1)}\Big)\text{dim}(k-1,0,1,1)\nonumber\\
&+s_1\Big(\sqrt{(\fft{k}{2}+3)(\fft{k}{2}+2)}\Big)\text{dim}(k-2,1,0,0)\nonumber\\
&+s_{\fft32}\Big(\fft{k+5}{2}-\fft32\Big)\text{dim}(k,0,0,1)+s_{\fft32}\Big(\fft{k+7}{2}-\fft32\Big)\text{dim}(k-1,0,1,0)\nonumber\\
&+s_2\Big(\sqrt{(\fft{k}{2}+3)\fft{k}{2}}\Big)\text{dim}(k,0,0,0) \, , 
\end{align}
%
where we have introduced the functions
%
\begin{equation}
\begin{split}
s_0(x)&=\fft{1}{288}(x^2+2)^2\,,\\
s_{\fft12}(x)&=-\fft{1}{144}x^2(x^2-2)\,,\\
s_1(x)&=\fft{1}{288}(4-12x^2+3x^4)\,,\\
s_{\fft32}(x)&=-\fft{1}{72}(11-8x^2+x^4)\,,\\
s_2(x)&=\fft{5}{288}(8-8x^2+x^4)\,.
\end{split}\label{s:spins}
\end{equation}
%
Remarkably, we again find a perfect cancellation
\begin{equation}
b_1(k) = 0 \, ,
\end{equation}
implying that the total heat kernel coefficient $b_1^{\text{tot}} = \sum_k b_1(k) = 0$.


%%%%%%%%%%%%%%%%%%%%%%%%
\subsection{KK supergravity on $S^7/\mathbb{Z}_k$}
\label{App:KK:S7modk}
%%%%%%%%%%%%%%%%%%%%%%%%


In the notation of \cite{Cordova:2016emh}, the $\mathcal{N}=8$ supermultiplet whose field content is given in Tables~\ref{tab:S7} and~\ref{tab:S7-m} is denoted by
\begin{equation}
B_1[0]^{(n+2,0,0,0)}_{\frac{n}{2}+1} \, .
\end{equation}
Note that we temporarily change notation and denote the KK level by $n \geq 0$ to reserve the notation $k$ for the order of the orbifold action $\mathbb{Z}_k$, as is common in the literature.

The spectrum of 11d supergravity compactified on $S^7/\mathbb{Z}_k$ can be obtained from the spectrum of the $S^7$ compactification as follows. First, we use the $\mathfrak{so}(8)\to\mathfrak{so}(6)\oplus\mathfrak{u}(1)$ branching rule~\cite{Liu:2016dau}
%
\begin{equation}
B_1[0]_{\fft{n}{2}+1}^{(n+2,0,0,0)}=B_1[0]_{\fft{n}{2}+1,-n-2}^{(0,0,n+2)}\oplus B_1[0]_{\fft{n}{2}+1,n+2}^{(0,n+2,0)}\oplus\sum_{i=0}^nB_1[0]_{\fft{n}{2}+1,-n+2i}^{(0,i+1,n-i+1)}\,,\label{N=8to6}
\end{equation}
%
where the subscripts on the right-hand side denote the scaling dimension of the primary in the given representation and the U(1) charge, respectively, and the superscripts are the SO(6) Dynkin label $(a,b,c)$. We must then select the multiplets that are stable under the orbifold action, i.e. the multiplets whose U(1) charge is divisible by $k$ \cite{Liu:2016dau}.\footnote{Here we choose the periodic spin structure on $S^7/\mathbb{Z}_k$ in order to impose the same constraint on the bosonic and fermionic modes, see \cite{Bobev:2021wir} for details.} In addition, we only keep the multiplets for which $n$ is even, see~\cite{Bobev:2021wir}. As a result, the  supermultiplets that make up the $\mathcal{N}=6$ KK spectrum are those of the form
\begin{equation}
B_1[0]_{h,-2r}^{(0,h-r,h+r)} \qquad \text{with} \quad h-|r|\geq0 \quad \text{and}\quad k\,|\,2r \,,\label{N=6:spectrum}
\end{equation}
where we have defined $h = \frac{n}{2} + 1 \in \mathbb{N}$ and $r = h - i - 1$ with $0\leq i \leq n$. The field content of these supermultiplets can be read off from \cite{Liu:2016dau}. Note that to obtain the correct field content for the special cases $0 \leq h - |r| \leq 3$, one must use the Racah-Speiser algorithm (reviewed e.g. in Appendix A.3 of \cite{Cordova:2016emh}). We will omit the details here and proceed to compute the heat kernel coefficients $(a_E,c,b_1)$ based on the KK spectrum~\eqref{N=6:spectrum}.

The SO(6) Weyl dimension formula for a representation with Dynkin label $(a,b,c)$ is
%
\begin{equation}
\dim(a,b,c)=\fft{1}{12}(1+a)(1+b)(1+c)(2+a+b)(2+a+c)(3+a+b+c)\,.\label{Weyl:dim:so(6)}
\end{equation}
%
Using this with the field content of the KK spectrum just discussed, we can proceed in the same way as in Appendix~\ref{App:KK:S7}. For the $(c,b_1)$ heat kernel coefficients, we find a perfect cancellation at any allowed given value of the quantum numbers $(h,r)$,
\begin{equation}
c(h,r) = b_1(h,r) = 0 \, .
\end{equation}
For the $a_E$ coefficient, we obtain a non-vanishing result:
\begin{equation}
a_E(h,r) = \fft{1}{24}(1+2h)\Big(h(1+h)(-4+5h+5h^2)+(7-10h-10h^2)r^2+5r^4\Big) \, .
\end{equation}
We discuss the sum over the spectrum in more details in Section~\ref{sec:KK-S7-k}.


%%%%%%%%%%%%%%%%%%%%%%%%
\subsection{KK supergravity for mABJM}
\label{App:KK:mABJM}
%%%%%%%%%%%%%%%%%%%%%%%%


Here we provide some details on the calculation of the SdW coefficient for the KK modes of the AdS$_4$ solution of 11d supergravity holographically dual to the mABJM SCFT. Since this background preserves $\mathcal{N}=2$ superconformal symmetry, we first present a short summary of the relevant superconformal multiplets. To facilitate the comparison with the literature we provide a map between superconformal multiplets in the supergravity conventions of Appendix A in \cite{Klebanov:2008vq} and the SCFT conventions of Table 4 in \cite{Cordova:2016emh}:
%
\begin{equation}
\begin{split}
A_1\bar{A}_1[2]_{\Delta=2}^{(r=0)}\quad&\leftrightarrow\quad \text{MGRAV}\,,\\
L\bar{A}_1[2]_{r+2}^{(r>0)}\quad&\leftrightarrow\quad \text{SGRAV with the upper sign}\,,\\
A_1\bar{L}[2]_{-r+2}^{(r<0)}\quad&\leftrightarrow\quad \text{SGRAV with the lower sign}\,,\\
L\bar{L}[2]_{\Delta>|r|+2}^{(r)}\quad&\leftrightarrow\quad \text{LGRAV}\,,\\
L\bar{A}_1[1]^{(r>0)}_{r+\fft32}\quad&\leftrightarrow\quad \text{SGINO with the upper sign}\,,\\
A_1\bar{L}[1]^{(r<0)}_{-r+\fft32}\quad&\leftrightarrow\quad \text{SGINO with the lower sign}\,,\\
L\bar{L}[1]_{\Delta>|r|+\fft32}^{(r)}\quad&\leftrightarrow\quad \text{LGINO}\,,\\
A_2\bar{A}_2[0]_{\Delta=1}^{(r=0)}\quad&\leftrightarrow\quad \text{MVEC}\,,\\
L\bar{A}_2[0]_{r+1}^{(r>0)}\quad&\leftrightarrow\quad \text{SVEC with the upper sign}\,,\\
A_2\bar{L}[0]_{-r+1}^{(r<0)}\quad&\leftrightarrow\quad \text{SVEC with the lower sign}\,,\\
L\bar{L}[0]_{\Delta>|r|+1}^{(r)}\quad&\leftrightarrow\quad \text{LVEC}\,,\\
L\bar{B}_1[0]^{(r>\fft12)}_{\Delta=r}~\&~A_2\bar{B}_1[0]^{(r=\fft12)}_{\Delta=r}\quad&\leftrightarrow\quad \text{HYP with the upper sign}\,,\\
B_1\bar{L}[0]^{(r<-\fft12)}_{\Delta=-r}~\&~B_1\bar{A}_2[0]^{(r=-\fft12)}_{\Delta=-r}\quad&\leftrightarrow\quad \text{HYP with the lower sign}\,.
\end{split}
\end{equation}
%
Note that the multiplets in \cite{Klebanov:2008vq} are labeled by their energy $E_0$, R-symmetry charge $y_0$, and the half-integer Lorentz spin $s_0$. The map to the corresponding quantities in \cite{Cordova:2016emh} is given by 
%
\begin{equation}
(E_0,y_0,s_0)~~ \longleftrightarrow~~ (\Delta,r,j/2)\,.
\end{equation}
%
We can use the explicit content of each of the multiplets above together with the information in Table~\ref{tab:coeffs} to systematically calculate the heat kernel coefficients for each superconformal multiplet. The result of this analysis is summarized in Table~\ref{HeatKernelCoefficientsMultiplets}. We hasten to note that the long superconformal multiplets have the interesting feature that while the individual states in the multiplet have heat kernel coefficients that depend on the conformal dimension (or mass in AdS) the total coefficients after summing over all fields in the multiplet are independent of this continuous parameter. The same is true for the $a_E$ and $c$ coefficients of short multiplets. The $b_1$ coefficient of short multiplets appears to depend on the conformal dimension, however one should bear in mind that for such multiplets the conformal dimension is uniquely determined by the spin and R-charge of the state.
%
\begin{table}[h]
	\centering \small 
	\renewcommand{\arraystretch}{1.5}
	\begin{tabular}{|c|c|c|c|} \hline
		& $a_E$ & $c$ & $b_1$  \\ \hline
		LGRAV & $\frac{5}{4}$ & $\frac{3}{4}$ & $\frac{1}{8}$\\ \hline
		SGRAV & $\frac{71-10\delta_{y_0,0}}{48}$ & $\frac{35-4\delta_{y_0,0}}{24}$ & $- \frac{1}{144} [3(E_0^2+2 E_0-11) + 2(E_0^3-3 E_0^2-9 E_0+25)\delta_{y_0,0}]$ \\ \hline
		MGRAV & $\frac{41}{24}$ & $\frac{13}{6}$ & 0\\ \hline
		LGINO & 0 & $-\frac{1}{2}$ & $-\frac{1}{12}$\\ \hline
		SGINO & $- \frac{11 + \delta_{y_0, 0}}{48}$ & $ - \frac{17 + \delta_{y_0, 0}}{24}$ & $ \frac{1}{2304}[ 48E_0(E_0+1)-276 - (2E_0 - 7)^2 (4E_0(E_0-1)-7)\delta_{y_0,0}] $\\ \hline
		LVEC & $\frac{1}{4}$ & $\frac{1}{4}$ & $\frac{1}{24}$ \\ \hline
		SVEC & $\frac{165 - 2 \delta_{y_0, 0}}{720}$ & $\frac{25-\delta_{y_0,0}}{120}$ & $ - \frac{1}{288}[6(E_0^2 -2) + (3 E_0^4-6 E_0^3-9 E_0^2+12 E_0+4) \delta_{y_0,0}] $\\ \hline
		MVEC & $\frac{5}{24}$ & $\frac{1}{6}$ & 0\\ \hline
		HYP & $\frac{1}{48}$ & $\frac{1}{24}$ & $ \frac{1}{48}(E_0 - 1)^2 $\\ \hline
	\end{tabular}
	\caption{The heat kernel coefficients $(a_E,c,b_1)$ for different $\cN = 2$ superconformal multiplets. The value of $E_0$ for each short multiplet is uniquely determined by the Lorentz spin and R-charge of its primary state. Note that some of the short multiplets do not include certain $y_0 = 0$ states which explains the appearance of the Kronecker in some of the expressions. The usual massless vector and hypermultiplets of matter-coupled 4d $\mathcal{N}=2$ gauged supergravity are MVEC and HYP, respectively.\label{HeatKernelCoefficientsMultiplets}}
\end{table}
%

After this general discussion we are ready to focus our attention on the specific AdS$_4$ $\mathcal{N}=2$ vacuum of interest. This solution was found long ago by Warner as a critical point of the potential of the 4d $\mathcal{N}=8$ ${\rm SO}(8)$ gauged supergravity \cite{Warner:1983vz} and then uplifted to a solution of 11d supergravity in \cite{Corrado:2001nv} and we will thus refer to this background as the CPW solution. A notable feature of this solution is that it has an ${\rm SU}(3) \times {\rm U}(1)$ symmetry in the internal space where the ${\rm U}(1)$ corresponds to the R-symmetry in the dual mABJM SCFT while ${\rm SU}(3)$ corresponds to its flavor symmetry. The KK spectrum of the short superconformal multiplets for this background was described in \cite{Klebanov:2008vq}, the spectrum of spin-2 KK modes was computed in \cite{Klebanov:2009kp}, while the full KK spectrum was analyzed in \cite{Malek:2020yue}.

Although there is no clear a priori notion of a ``KK level'' for the spectrum of 11d supergravity AdS$_4$ solutions one can use the fact that the CPW solution is related to AdS$_4 \times S^7$ by a supersymmetric domain wall and use the integer $k$ labelling the $\mathcal{N}=8$ KK spectrum in Table~\ref{tab:S7-m} as giving some notion of a ``KK level''. To avoid confusion and make it clear we refer to the KK spectrum of the CPW solution we will call this integer $n$ below. With this at hand one can compactly summarize the KK spectrum using the results of \cite{Malek:2020yue} as follows
%  
\begin{equation}
\label{E0U3}
\begin{split}
{\rm GRAV:}\quad E_0 =&\; \frac{1}{2} + \sqrt{\frac{9}{4} + \frac{1}{2}n(n+6) - \frac{4}{3}C_{p,q} + \frac{1}{2}\Bigl(r + \frac{2}{3}(q-p)\Bigr)^2 } \, ,\\[1mm]
{\rm GINO:}\quad E_0 =&\; \frac{1}{2} + \sqrt{\frac{7}{2} + \frac{1}{2}n(n+6) - \frac{4}{3}C_{p,q} + \frac{1}{2} r^2} \, ,\\[1mm]
{\rm VEC/HYP:}\quad E_0 =&\; \frac{1}{2} + \sqrt{\frac{17}{4} + \frac{1}{2}n(n+6) - \frac{4}{3}C_{p,q} + \frac{1}{2}r^2} \, ,
\end{split}
\end{equation}
%
where
\begin{equation}
C_{p,q} = \frac{1}{3}(p^2 + q^2 + pq) + p + q \, .
\end{equation}
Here the integers $[p,q]$ specify the Dynkin labels of the ${\rm SU}(3)$ representation of the given multiplet and $C_{p,q}$ is its quadratic Casimir.\\

The data about the KK spectrum not captured by the information presented above is which ${\rm SU}(3)$ representation precisely are contained in the spectrum. For the short multiplets this was systematically studied in \cite{Klebanov:2008vq,Malek:2020yue}, see in particular Table 6 in \cite{Klebanov:2008vq} and Equation (5.99) in \cite{Malek:2020yue}.\footnote{Note that the relevant case for our discussion was dubbed Scenario I in \cite{Klebanov:2008vq}.} For each non-negative integer $n$ the list of short multiplets is summarized in Table~\ref{ShortMultiplets} where we also present their ${\rm SU}(3)$ Dynkin labels.
%
\begin{table}[h]
	\renewcommand{\arraystretch}{1.5}
	\centering
	\begin{tabular}{|c|c|} \hline
		SGRAV/MGRAV & $[0,0]_{\pm n}$ \\ \hline
		SGINO & $[n+1,0]_{\frac{n+1}{3} },\ [0, n+1]_{-\frac{n+1}{3}}$ \\ \hline
		SVEC/MVEC & $[n+1,1]_{\frac{n}{3} },\ [1, n+1]_{-\frac{n}{3}}$ \\ \hline
		HYP & $[n+2,0]_{\frac{n+2}{3} },\ [0, n+2]_{-\frac{n+2}{3}}$ \\ \hline
	\end{tabular}
	\caption{The list of short multiplets in the KK spectrum of the CPW solution along with their ${\rm SU}(3)$ Dynkin labels. Note that $n\geq 0$ and when $n = 0$, the SGRAV and SVEC multiplets reduce to a single MGRAV and MVEC multiplet, respectively.\label{ShortMultiplets}}
\end{table}
%
Using this information together with the SU(3) Weyl dimension formula
\begin{equation}
\dim(p,q)=\fft12(p+1)(q+1)(p+q+2)\,,\label{Weyl:SU(3)}
\end{equation}
and the heat kernel coefficients in Table~\ref{HeatKernelCoefficientsMultiplets}, we find the following list of $(a_E,c,b_1)$ coefficients for all short multiplets at fixed KK level $n$, 
%
\begin{align}
\label{eq:HK-mABJM-short}
{\rm S/MGRAV:} \quad &\;a_E(n) = \frac{71}{24} - \frac{5}{4}\delta_{n,0} \, , \quad c(n) = \frac{35}{12} - \frac{3}{4}\delta_{n,0} \, , \nonumber\\[1mm] 
&\; b_1(n) =- \frac{ n(n+6) - 3 }{24} - \frac{1}{8}\delta_{n,0} \, , \nonumber\\[1mm]
{\rm SGINO:} \quad &\;a_E(n) = -\frac{11}{48}(n+2)(n+3)\, , \quad c(n) = -\frac{17}{24}(n+2)(n+3) \, ,\nonumber\\[1mm]
&\;b_1(n) = \frac{1}{432}(n+2)(n+3)[n(n+14) - 5] \, , \\[1mm]
{\rm S/MVEC:} \quad &\;a_E(n) = \frac{11}{24}(n+2)(n+4) - 2\delta_{n,0}\, , \quad c(n) = \frac{5}{12}(n+2)(n+4) - 2\delta_{n,0} \, ,\nonumber\\[1mm]
&\;b_1(n) = - \frac{1}{216}(n+2)(n+4)[n(n+6) - 9] -  \frac{1}{3}\delta_{n,0}\, , \nonumber\\[1mm]
{\rm HYP:} \quad &\;a_E(n) = \frac{1}{48}(n+3)(n+4) \, , \quad c(n) = \frac{1}{24}(n+3)(n+4) \, ,\nonumber\\[1mm]
&\;b_1(n) = \frac{1}{432}(n+3)(n+4)(n-1)^2 \, .\nonumber
\end{align}
%

We now move on to discuss the long multiplets. Here the situation is more involved and it is harder to obtain compact expressions for the total number of long multiplets, i.e. to sum over the corresponding ${\rm SU}(3)$ representation labels. To make progress we can use the strategy employed in \cite{Nicolai:1985hs,Klebanov:2008vq,Malek:2020yue,Cesaro:2020piw}. Namely we can rely on the fact that the CPW solution is connected by a holographic RG flow to the AdS$_4\times S^7$ background and thus we can use the symmetry breaking pattern from the $\mathcal{N}=8$ supersymmetry with ${\rm SO}(8)$ R-symmetry in the UV to $\mathcal{N}=2$ supersymmetry with ${\rm U}(1)$ R-symmetry and ${\rm SU}(3)$ flavor symmetry in the IR to organize the multiplets.\footnote{We have independently confirmed the calculations in \cite{Nicolai:1985hs,Klebanov:2008vq,Malek:2020yue,Cesaro:2020piw} using results from \cite{Slansky:1981yr} as well as the LieART package \cite{Feger:2019tvk}. We note that there are probably some typos in \cite{Klebanov:2008vq}, namely in Table 18, there should be two LGINO 0 in the $[1,1]$ representation and in Table 19 there should be two LVEC 0 in the $[0,0]$ representation.} Below we present explicit expressions for the total number of long multiplets at KK level $n$ and a short summary on how they are obtained. Since the heat kernel coefficients  $(a_E,c,b_1)$ are constant for all long multiplets, see Table~\ref{HeatKernelCoefficientsMultiplets}, this counting is sufficient for our purposes.\\

{\bf LGRAV:} It was observed in \cite{Malek:2020yue} that at level $n$, the graviton multiplets transform under SU(3)$\times$U(1)$_R$ as follows:
\begin{equation} \label{mABJMLGRAV}
[p, q]_{ \frac{p-q}{3} + (a-b) }\, ,\quad \forall\;p,q,a,b\in \mathbb{N} \,, \;\;\text{with}\;\; p + q + a + b = n \, .
\end{equation}
Thus we only need to count the ordered partition $(p,q,a,b)$ of the integer $n$; which is $n+1-p-q$ for fixed $p,q$.  Na\"ively, the total number of LGRAV multiplets is then obtained by summing over $p$ and $q$ to find
%    
\begin{equation}
\sum_{\substack{p,q = 0 \\ p+q\leq n}} (n+1-p-q) \dim(p,q) = \frac{1}{360} (n+1) (n+2) (n+3)^2 (n+4)(n+5) \, .
\end{equation}
%
This result is true except for $p = q = 0$ and $(a,b) = (n,0)$ or $(0,n)$, where the multiplets are short(or massless when $n=0$), thus the corrected weighted sum that gives the total number of LGRAV multiplets at KK level $n$ is:
%
\begin{equation}
\Omega^{\rm{LGRAV}}(n) =  \frac{1}{360} (n+1) (n+2) (n+3)^2 (n+4)(n+5) - (2 - \delta_{n,0}) \, .
\end{equation}
%

{\bf LGINO:} The analysis for the LGINO multiplet is more complicated since there is no compact formula analogous to \eqref{mABJMLGRAV}. As explained above we circumvent this difficulty by using the fact that the field content of the mABJM theory is inherited from the $\mathcal{N} = 8$ multiplets of the ABJM theory. This implies that for a given level $n$, the number of particles with the same spin is identical. The number of LGINO multiplets is thus equal to the number of spin-3/2 fields, minus those in L/SGRAV and SGINO multiplets. The total number of spin-3/2 fields is dictated by the following ${\rm SO}(8)$ representations:
%
\begin{equation}
\begin{aligned}
\dim(n,0,0,1) &= \frac{1}{90} (n+1) (n+2) (n+3) (n+4) (n+5) (n+6) \, ,\\
\quad \dim(n-1,0,1,0) &= \frac{1}{90} n (n+1) (n+2) (n+3) (n+4) (n+5) \, .
\end{aligned}
\end{equation}
%
The number of spin-3/2 particles in the graviton multiplets is:
%
\begin{equation}
4\Bigl[\frac{1}{360} (n+1) (n+2) (n+3)^2 (n+4)(n+5) - (2 - \delta_{n,0})\Bigr] + 6(1-\delta_{n,0}) + 2\delta_{n,0} \, .
\end{equation}
% 
The number of spin-3/2 particles in the two SGINO multiplets is $2 \times \dim(n+1,0) = (n+2)(n+3)$. With this at hand we finally find the total number of LGINO multiplets:
% 
\begin{equation}
\Omega^{\rm LGINO}(n) =  \frac{1}{90}n(n+1)(n+4)(n^3+13 n^2+61 n+123) \, .
\end{equation}
%



{\bf LVEC:} To find the total number of LVEC multiplets we follow the same approach as above. First, we find the total number of spin-1 modes from the ${\rm SO}(8)$ representations:
%
\begin{equation}
\begin{aligned}
&\dim(n,1,0,0) + \dim(n-1, 0, 1,1)_{n \ge 1} + \dim(n-2,1,0,0)_{n\ge 2} \\ 
&\quad = \frac{3}{40}(n+1)(n+2)(n+3)^2(n+4)(n+5) + \delta_{n,0} \, .
\end{aligned}
\end{equation}
% 
The number of spin-1 modes contained in LGRAV and SGRAV/MGRAV is
%
\begin{equation}
6\Bigl[\frac{1}{360} (n+1) (n+2) (n+3)^2 (n+4)(n+5) - (2 - \delta_{n,0})\Bigr] + 6(1-\delta_{n,0}) + \delta_{n,0} \, ,
\end{equation}
% 
while the number contained in LGINO and SGINO is
% 
\begin{equation}
4\Bigl[\frac{1}{90}n(n+1)(n+4)(n^3+13 n^2+61 n+123)\Bigr] + 6\dim(n+1,0) \, .
\end{equation}
%   
Finally the number of spin-1 modes in SVEC/MVEC multiplets is
%
\begin{equation}
2 (1-\delta_{n,0}) \dim(n+1,1) + \delta_{n,0} \dim(1,1) \, . 
\end{equation}
%  
Combining all this we find that the total number of LVEC multiplets at KK level $n$ is
%
\begin{equation}
\Omega^{\rm LVEC}(n) =  \frac{1}{72}(n+3)(n+4) (n^4+11 n^3+41 n^2+61 n-42) + 8 \delta_{n,0} \, .
\end{equation}
%

We now have the total number of each type of long and short multiplets in the KK spectrum of the CPW background. We can combine this with the information in Table~\ref{HeatKernelCoefficientsMultiplets} to find the total heat kernel coefficients. A short calculation shows that, at each KK level $n$, we find a perfect cancellation for the $c$ coefficient:
\begin{equation}
c(n) = \frac34\Omega^{\rm{LGRAV}}(n) - \frac12\Omega^{\rm{LGINO}}(n) + \frac14\Omega^{\rm{LVEC}}(n) + c^{\text{short}}(n) = 0 \, ,
\end{equation}
where $c^{\text{short}}$ is the sum of all $c(n)$ in the short sector~\eqref{eq:HK-mABJM-short}. The same cancellation occurs for the $b_1$ coefficient:
\begin{equation}
b_1(n) = \frac18\Omega^{\rm{LGRAV}}(n) - \frac1{12}\Omega^{\rm{LGINO}}(n) + \frac1{24}\Omega^{\rm{LVEC}}(n) + b_1^{\text{short}}(n) = 0 \, .
\end{equation}
Lastly, for the $a_E$ coefficient, we obtain the following compact final result,
%
\begin{equation}
\begin{split}
a_E(n) =&\; \frac{5}{4}\Omega^{\rm LGRAV}(n) + \frac{1}{4} \Omega^{\rm LVEC}(n) + a_E^{\text{short}}(n) \\[1mm]
=&\; \frac{1}{144} (n+1)(n+2)(n+3)^2 (n+4)(n+5) \, .
\end{split}
\end{equation}
%    
Notably, these are exactly the same expressions we found for the heat kernel coefficients of the KK spectrum of the $\mathcal{N}=8$ AdS$_4\times S^7$ background in \eqref{S7:a:bulk}, \eqref{S7:c:bulk}, and \eqref{S7:b:bulk}. The calculation leading to these results for the two distinct 11d supergravity backgrounds is very different and as we discuss in the main text it will be interesting to obtain further insights into why the results end up the same. Regardless, it is clear that the total $c$ and $b_1$ coefficients after summing over $n$ vanish. The total $a_E$ heat kernel coefficient takes the form of a divergent sum which is identical to the one encountered in the AdS$_4\times S^7$ and thus should be regularized in the same way.


%%%%%%%%%%%%%%%%%%%%%%%%
\subsection{KK supergravity on $N^{0,1,0}$}
\label{App:KK:N010}
%%%%%%%%%%%%%%%%%%%%%%%%


The KK supergravity spectrum of the AdS$_4\times N^{0,1,0}$ 11d supergravity solution was presented in \cite{Fre:1999gok} where it was organized into multiplets of the ${\rm OSp}(3|4)$ superconformal algebra and the ${\rm SU}(3)$ flavor symmetry. We will use both the conventions of \cite{Fre:1999gok} and \cite{Cordova:2016emh} when we discuss our results. The map between the two sets of conventions is given by
%
\begin{equation}
(E_0,J_0,s_0)~~ \longleftrightarrow~~ (\Delta,R/2,j/2) \,,
\end{equation}
%
where $\Delta\in\mathbb Z/2$ is the conformal dimension, $R\in\mathbb Z_{\geq0}$ denotes the ${\rm SO}(3)$ $R$-symmetry representation, and $j\in\mathbb Z_{\geq0}$ is the Lorentz spin. Note that the dimension of the ${\rm SO}(3)$ representation with label $R$ is given by $\text{dim}(R)=R+1$ and analogously the dimension of the Lorentz spin-$j$ representation is $\text{dim}(j)=j+1$.

The complete list of 3d $\mN=3$ multiplets can be found in Table 5 of \cite{Cordova:2016emh} and is summarized in Table~\ref{table:N010}.
%
\begin{table}[h]
	\centering
	\renewcommand{\arraystretch}{1.5}
	\begin{tabular}{|c|c|c|}
		\hline
		name & primary & unitarity bound\\\hline
		$L$ & $[j]_\Delta^{(R)}$ & $\Delta>\fft12j+\fft12R+1$ \\\hline
		$A_1$ & $[j]_\Delta^{(R)}~~(j\geq1)$ & $\Delta=\fft12j+\fft12R+1$ \\\hline
		$A_2$ & $[0]_\Delta^{(R)}$ & $\Delta=\fft12R+1$ \\\hline
		$B_1$ & $[0]_\Delta^{(R)}$ & $\Delta=\fft12R$ \\\hline
	\end{tabular}\caption{The complete list of $\mN=3$ multiplets\label{table:N010}}
\end{table}
%
The $\mN=3$ multiplets arising from the $N^{0,1,0}$ KK spectrum discussed in \cite{Fre:1999gok} read
%
\begin{equation}
\begin{split}
L[1]_\Delta^{(R)}\quad&\leftrightarrow\quad SD(s_\text{max}=2,E_0>J_0+3/2,J_0|3)\,,\\
L[0]_\Delta^{(R)}\quad&\leftrightarrow\quad SD(s_\text{max}=3/2,E_0>J_0+1,J_0|3)\,,\\
A_1[1]_\Delta^{(R)}\quad&\leftrightarrow\quad SD(s_\text{max}=2,E_0=J_0+3/2,J_0|3)\,,\\
A_2[0]_\Delta^{(R)}\quad&\leftrightarrow\quad SD(s_\text{max}=3/2,E_0=J_0+1,J_0|3)\,,\\
B_1[0]_\Delta^{(R)}\quad&\leftrightarrow\quad SD(s_\text{max}=1,E_0=J_0,J_0|3)\,,
\end{split}
\end{equation}
%
where on the right hand side we used the notation of \cite{Fre:1999gok}. The descendants for generic multiplets and conserved current multiplets are presented in Section 4.3 and 5.4.3 of \cite{Cordova:2016emh}, respectively (see also Table 1-5 of \cite{Fre:1999gok}). Note that the $A_2[0]_\Delta^{(0)}$ multiplet is not present in the spectrum since it contains an extra supercurrent multiplet not present for the AdS$_4\times N^{0,1,0}$ solution which is genuinely $\mathcal{N}=3$ supersymmetric.

To obtain Tables 1-5 of \cite{Fre:1999gok} from the generic expressions given in Section 4.3 of \cite{Cordova:2016emh}, one needs to use the Racah-Speiser (RS) algorithm. For the $\mathfrak{so}(3)$ Lie algebra of Lorentz spin, the RS algorithm is simply given as
%
\begin{equation}
[j]^{(R)}=\begin{cases}
0 & (j=-1) \\
-[-j-2]^{(R)}& (j=-2,-3,\cdots)
\end{cases}\qquad(R\geq0)\,,
\end{equation}
%
where the overall minus sign on the right-hand side means that it ``eats'' the representation without the minus sign. Since the $R$-symmetry is also controlled by the same algebra, we can apply the same rule, i.e.
%
\begin{equation}
[j]^{(R)}=\begin{cases}
0 & (R=-1) \\
[j]^{-(-R-2)}& (R=-2,-3,\cdots)
\end{cases}\qquad(j\geq0)\,,
\end{equation}
%
with the same interpretation for the overall minus sign in the superscript of the RHS.

To calculate the heat kernel coefficients of each $\mathcal{N}=3$ superconformal multiplet of interest, we need to add up the coefficients of every field in the multiplet and use the values in Table~\ref{tab:coeffs}. The result for each of the multiplets in Table~\ref{table:N010} is summarized below.\footnote{Note that the rightmost entry of Table 5 of \cite{Fre:1999gok} is missing one of the two spin-$\fft12$ representations.}
\begin{align} \label{eq:HKEN3Multiplets}
L[1]_\Delta^{(R)} \;\text{with}\;\Delta>\tfrac12 R + \tfrac32: \quad &a_E(R) = \fft{3(1+R)}{2} \, , \quad c(R) = 0 \, , \quad b_1(R) = 0 \, , \nonumber\\[1mm]
L[0]_\Delta^{(R)} \;\text{with}\;\Delta>\tfrac12 R+1: \quad &a_E(R) = \fft{1+R}{2} \, , \quad c(R) = 0 \, , \quad b_1(R) = 0 \, , \nonumber\\[1mm]
A_1[1]_\Delta^{(R)} \;\text{with}\;\Delta=\tfrac12 R+\tfrac32: \quad &a_E(R) = \fft{5(1+R)}{4} \, , \quad c(R) = \frac{5+R}{4} \, , \quad b_1(R) = 0 \, , \nonumber\\[1mm]
A_2[0]_\Delta^{(R)} \;\text{with}\;\Delta=\tfrac12 R+1: \quad &a_E(R) = -\fft{(1-R)}{4} \, , \quad c(R) = -\frac{3+R}{4} \, , \quad b_1(R) = 0 \, , \nonumber\\[1mm]
B_1[0]_\Delta^{(R)} \;\text{with}\;\Delta=\tfrac12 R: \quad &a_E(R) = \begin{cases} -\fft{1-R}{4} & R\geq2 \\ \fft{1+12R}{360} & R=0,1\end{cases} \, , \\[1mm]  
&c(R) =\begin{cases} -\fft{1-R}{4} & R\geq2 \\ \fft{1+7R}{120} & R=0,1 \end{cases} \, , \quad b_1(R) = 0 \, .\nonumber
\end{align}
Then the total heat kernel coefficients are obtained after summing over all multiplets in the KK tower while taking into account their SU(3) representations. This can be done using the dimension formula~\eqref{Weyl:SU(3)}.

Since all $\mathcal{N}=3$ multiplets have vanishing $b_1(R)$, we immediately get that
%
\begin{equation}
b_1^\text{tot}=0 \, .
\end{equation}
%
Next we consider the total heat kernel coefficient $c^\text{tot}$. Since the $L[j]_\Delta^{(R)}$ long multiplets have vanishing $c$ coefficients, we only need to consider the $A_{1,2}$ and $B_{1}$ short multiplets and their flavor representations given in Sections 3.2 and 3.3 of \cite{Fre:1999gok}. For example, the massive short graviton multiplet $A_1[1]_\Delta^{(R)}$ falls in SU(3) representations with Dynkin label $(k,k)$ with $k\geq 1$, and the R-charge is given by $R=2k$. In addition, there is a massless graviton multiplet in the $(0,0)$ representation with $R=0$. Therefore, the short graviton sector contributes to the $c$ coefficient with
\begin{equation}
c^{\text{short}(2)} = \sum_{k=0}^\infty\dim(k,k)\fft{5+2k}{4} = \fft14\sum_{k=0}^\infty(1+k)^3(5+2k) \, .
\end{equation}
The massive short gravitino multiplet $A_2[0]_\Delta^{(R)}$ falls in the $(k,k+3)$ representation with $k\geq 0$. In addition, we must consider the conjugate representation $(k+3,k)$ to obtain the complete spectrum. The R-charge is fixed to $R = 2(k + 1)$ and the short gravitino sector contributes to the $c$ coefficient with
\begin{equation}
\label{eq:ciiiN010}
\begin{split}
c^{\text{short}(3/2)} =&\; \sum_{k=0}^\infty[\dim(k,k+3)+\dim(k+3,k)]\fft{-3-2(k+1)}{4} \\
=&\; -\fft14\sum_{k=0}^\infty(1+k)(4+k)(5+2k)^2 \, .
\end{split}
\end{equation}
The massive short vector multiplet $B_1[0]_\Delta^{(R)}$ falls in the $(k,k)$ representation with $k \geq 2$, and with $R = 2k$. Together with the massless vector multiplet in the $(1,1)$ representation with $R=2$, this gives 
\begin{equation}
c^{\text{short}(1)} = \sum_{k=0}^\infty\dim(k+1,k+1)\fft{-1+2(k+1)}{4} = \fft14\sum_{k=0}^\infty(2+k)^3(1+2k) \, .
\end{equation}
Lastly, the (massless) Betti multiplet is in the $(0,0)$ SU(3) representation and has $R=2$, for a contribution of
\begin{equation}
c^{\text{Betti}} = \dim(0,0)\fft{-1+2}{4}=\fft14 \, .
\end{equation}
We should now regularize all the above infinite series. In Appendix~\ref{app:reg}, we present a regularization method adapted from~\cite{friedman2012special}. However, this method is based on zeta-function regularization and is therefore not stable. This means that we will obtain different results depending on whether we first sum all short sector contributions and regularize the resulting series, or if we regularize each short sector separately before taking the sum. By doing the former, we find that $c^{\text{tot}} \neq 0$, in violation of our bootstrap constraints~\eqref{eq:no-Cloc}. However, we do find a remarkable cancellation if we decide to regulate each series independently. Our regularization prescription based on~\eqref{eq:FP-zeta-reg} attaches the following finite values:
\begin{equation}
\label{eq:c-N010-reg}
c^{\text{short}(2)} = \frac{55}{1024} \, , \qquad c^{\text{short}(3/2)} = -\frac12 \, , \qquad c^{\text{short}(1)} = \frac{201}{1024} \, ,
\end{equation}
and together with the Betti multiplet contribution, we arrive at
\begin{equation}
c^{\text{tot}} = 0 \, .
\end{equation}
Thus, it is possible to adopt a regularization prescription for the sum over the KK spectrum that is compatible with the bootstrap constraints~\eqref{eq:no-Cloc}. 

The calculation of the $a_E^\text{tot}$ coefficient is more subtle. First, we need to take into account the contributions from both long and short multiplets. Moreover, the resulting infinite sums involve multiple summation indices, which complicates the task of finding a suitable regularization. We give each contribution to $a_E^{\text{tot}}$ in turn below.

i) From Table (9) of \cite{Fre:1999gok}, we have
%
\begin{equation}
\label{eq:aE-N010-long}
\begin{split}
a_E^\text{i)}&=\sum_{k=0}^\infty\sum_{j\geq2}^{\infty}\text{dim}(k,k+3j)\sum_{J_0=j}^{k+j}\bigg[\fft{3(1+2J_0)}{2}+\fft{1+2J_0}{2}+\fft{1+2J_0}{2}\bigg]\\
&=\fft54\sum_{k=0}^\infty\sum_{j\geq2}^{\infty}(1+k)^2(1+2j+k)(1+3j+k)(2+3j+2k)\,.
\end{split}
\end{equation}

ii) From Table (10) of \cite{Fre:1999gok}, we have
%
\begin{equation}
\begin{split}
a_E^\text{ii)}&=\sum_{k=0}^\infty\text{dim}(k,k+3)\Bigg[\sum_{J_0=1}^{k+1}\bigg[\fft{3(1+2J_0)}{2}+\fft{1+2J_0}{2}\bigg]+\sum_{J_0=1}^{k}\fft{1+2J_0}{2}\Bigg]\\
&=\frac14\sum_{k=0}^\infty(1+k)(4+k)(5+2k)(12 + 18k + 5k^2) \, .
\end{split}
\end{equation}

iii) From Table (11) of \cite{Fre:1999gok}, we have
%
\begin{equation}
\begin{split}
a_E^\text{iii)}&=\sum_{k=0}^\infty\text{dim}(k,k)\Bigg[\sum_{J_0=0}^{k-1}\bigg[\fft{3(1+2J_0)}{2}+\fft{1+2J_0}{2}\bigg]+\sum_{J_0=0}^{k}\fft{1+2J_0}{2}\Bigg]\\
&= \frac12\sum_{k=0}^{\infty}(1+k)^3(1+2k+5k^2) \, .
\end{split}
\end{equation}

iv) From (12), (13) and (18), (19) of \cite{Fre:1999gok}, we have
%
\begin{equation}
a_E^{\text{short}(2)}=\sum_{k=0}^\infty\dim(k,k)\fft{5(1+2k)}{4}=\fft54\sum_{k=0}^\infty(1+k)^3(1+2k)\,.
\end{equation}

v) From (14), (15) of \cite{Fre:1999gok}, we have
%
\begin{equation}
a_E^{\text{short}(3/2)}=\sum_{k=0}^\infty\dim(k,k+3)\fft{-1+2(k+1)}{4}=\fft18\sum_{k=0}^\infty(1+k)(4+k)(1+2k)(5+2k)\,.
\end{equation}

vi) From (16), (17) and (20), (22) of \cite{Fre:1999gok}, we have
%
\begin{equation}
a_E^{\text{short}(1)}=\sum_{k=0}^\infty\dim(k+1,k+1)\fft{-1+2(k+1)}{4}=\fft14\sum_{k=0}^\infty(2+k)^3(1+2k)\,.
\end{equation}
% 

vii) From (21), (22) of \cite{Fre:1999gok}, we have
%
\begin{equation}
a_E^{\text{Betti}}=\dim(0,0)\fft{-1+2}{4}=\fft14\, .
\end{equation}

Since we do not have bootstrap constraints involving $a_E$, it is difficult to come up with the right prescription for regularizing the above sums. In addition, the method presented in Appendix~\ref{app:reg} does not apply to the long sector series~\eqref{eq:aE-N010-long} which involve both $k$ and $j$ quantum numbers.

	\subsection{$S^7/\mathbb{Z}_4$ theory with antiperiodic spin structure}
	
	For ABJM theory dual to AdS$_4\times S^7/\mathbb{Z}_k$, there is a special case $k=4$ where one can reverse the spin structure, i.e., take the anti-periodic spin structure. The resulting theory has been shown to have 3d $\cN = 2$ supersymmetries. \cite{Bobev:2021wir} 
	
	The coefficients for the minimally coupled antiperiodic theory are given by
	\begin{equation}
		(a_E^{\rm min})_0  = \frac{29}{6},\quad c_0^{\rm min} = \frac{14}{3},\quad (b_1^{\rm min})_0 = 0.
	\end{equation}
	For a general KK-level $k$, the multiplets are listed as in (3.7) of \cite{Bobev:2021wir}. The invariance of $\mathbb{Z}_4$ requires $k$ to be even. The shortening conditions are different whether or not $k$ is divisible by 4, which we need to treat seperatedly. Here is the result:
	\begin{itemize}
		\item {\bf Case I}: $k$ is divisible by $4$: \footnote{As a clarification of the notation, $k$ in the polynomials are the KK levels, while $k$ in the indices are the CS levels. }
		\begin{equation}
			\begin{aligned}
				(a_E)_k &= \frac{1}{288}(k+2)(k+3)(k+4)(k^3 + 9k^2 + 23k + 58),\\
				c_k &= \frac{7}{36} (k+2)(k+3)(k+4),\\
				(b_1)_k &= - \frac{1}{144}k (k+2)(k+3)(k+4) (k+6).\\
			\end{aligned}
		\end{equation}
		
		\item {\bf Case II}: $k$ not divisible by $4$:
		\begin{equation}
			\begin{aligned}
				(a_E)_k &= \frac{1}{288}(k+2)(k+3)(k+4)(k^3 + 9k^2 + 23k - 28),\\
				c_k &= -\frac{7}{36} (k+2)(k+3)(k+4),\\
				(b_1)_k &= \frac{1}{144}k (k+2)(k+3)(k+4) (k+6).\\
			\end{aligned}
		\end{equation}
		
		\item {\bf Case III}: $k$ is odd:
		\begin{equation}
			(a_E)_k = c_k = (b_1)_k = 0.
		\end{equation}
	\end{itemize}
	The coefficients above exactly reproduce the results based on the explicit multiplets listed in \cite{Bobev:2021wir} for $k = 2,4,6,8$. 
	
	Using the regularisation prescribed in \cite{friedman2012special}, we obtain:
	\begin{equation}
		\begin{aligned}
			\sum_k c_k &= \sum_{m=0} c_{4m} + \sum_{m=0} c_{4m+2} = - \frac{7}{320} + \frac{7}{320}  = 0,\\
			\sum_k (b_1)_k &= \sum_{m=0} (b_1)_{4m} + \sum_{m=0} (b_1)_{4m+2} = \frac{1565}{72576} -  \frac{1565}{72576} = 0,\\
		\end{aligned}
	\end{equation}
	with agree with our bootstrap constraint. As for $(a_E)_k$, we first re-write them as:
	\begin{equation}
		\begin{aligned}
			(a_E)_k &= (a_E^{\rm 0})_k + (\delta a_E)_k,\\
			&  (a_E^{\rm 0})_k = \left\{ \begin{array}{c}
				\frac{1}{288} (k+1)(k+2)(k+3)^2 (k+4)(k+5),\quad k \in 2 \mathbb{Z},\\
				0,\quad k \in 2 \mathbb{Z} + 1,\\
			\end{array}\right. \\
			& (\delta a_E)_k = \left\{ \begin{array}{c}
				\frac{43}{288}(k+2)(k+3)(k+4),\quad k \in 4\mathbb{Z},\\
				- \frac{43}{288}(k+2)(k+3)(k+4),\quad k  \in 4\mathbb{Z} + 2,\\
				0,\quad k \in 2 \mathbb{Z}+1.\\
			\end{array}  \right.
		\end{aligned}
	\end{equation}
	Here, $ (a_E^{\rm 0})_k $ is identical to a similar part of gauged supergravity with ordinary spin structure \cite{Bobev:2023dwx}. Thus, if the same regularization is applied, the difference $(\delta a_E)^{\rm tot}$ should give zero over summing over all KK modes similarly as $c^{\rm tot}$ and $(b_1)^{\rm tot}$.  
	%    {\bf Dictation of AdS/CFT:} From the field theory side, the matrix model doesn't care the value of $k$ (the CS level) and gives $ \frac{1}{4} \log N$. This requires:
	%    \begin{equation}
		%		\sum_{ k \in \mathbb{N}, k\ {\rm even}}  \frac{1}{288} (k+1)(k+2)(k+3)^2 (k+4)(k+5)  = \sum_{k \in \mathbb{N}}  \frac{1}{144} (k+1)(k+2)(k+3)^2 (k+4)(k+5).
		% \end{equation}
	
	\subsubsection{periodic spin structure and a puzzle (with solution)}
	The heat-kernel coefficients of these theories are already reviewed in Appendix D of \cite{Bobev:2023dwx}. We first review it for $k = 3$ and $4$, then give a general guess and then a puzzle raised by AdS/CFT. 
	
	The coefficients $c$ and $b_1$ vanish level-by-level, so our fucus will be $a_E$. For $k = 4$, the coefficients are:
	\begin{equation}
		\begin{aligned}
			(a_E^{k=4})_k &= (a_E^{\rm 0})_k + (\delta a_E)_k,\\
			&  (a_E^{\rm 0})_k = \left\{ \begin{array}{c}
				\frac{1}{288} (k+1)(k+2)(k+3)^2 (k+4)(k+5),\quad k \in 2 \mathbb{Z},\\
				0,\quad k \in 2 \mathbb{Z} + 1,\\
			\end{array}\right. \\
			& (\delta a_E)_k = \left\{ \begin{array}{c}
				\frac{1}{96}(k+2)(k+3)(k+4),\quad k \in 4\mathbb{Z},\\
				- \frac{1}{96}(k+2)(k+3)(k+4),\quad k  \in 4\mathbb{Z} + 2,\\
				0,\quad k \in 2 \mathbb{Z}+1.\\
			\end{array}  \right.
		\end{aligned}
	\end{equation}
	For $k = 3$, the coefficients are:
	\begin{equation}
		\begin{aligned}
			(a_E^{k=3})_k &= (a_E^{\rm 0})_k + (\delta a_E)_k,\\
			&  (a_E^{\rm 0})_k = \left\{ \begin{array}{c}
				\frac{1}{432} (k+1)(k+2)(k+3)^2 (k+4)(k+5),\quad k \in 2 \mathbb{Z},\\
				0,\quad k \in 2 \mathbb{Z} + 1,\\
			\end{array}\right. \\
			& (\delta a_E)_k = \left\{ \begin{array}{c}
				\frac{2}{27}(k+3)^2,\quad k \in 6\mathbb{Z},\\
				\frac{1}{27}(k+1)(k+3)(k+4),\quad k  \in 6\mathbb{Z} + 2,\\
				- \frac{1}{27}(k+1)(k+3)(k+4),\quad k  \in 6\mathbb{Z} + 4,\\
				0,\quad k \in 2 \mathbb{Z}+1.\\
			\end{array}  \right.
		\end{aligned}
	\end{equation}
	The KK-sum of $(\delta a_E)_k$ vanishes, so we only have the summation over $(a_E^0)_k$. It's natural to conjecture that 
	\begin{equation}
		\begin{aligned}
			(a_E^{k = p})_k &= \frac{1}{p'} \frac{1}{144} (k+1)(k+2)(k+3)^2 (k+4)(k+5) + (\delta a_E)_k,\\
			p' &\equiv \left\{ \begin{aligned}
				& p,\quad p \in 2\mathbb{Z}+1,\\
				& p/2, \quad p \in 2 \mathbb{Z}.\\
			\end{aligned}\right.
		\end{aligned}
	\end{equation}
	Let's denote:
	\begin{equation}
		\begin{aligned}
			\Sigma_{e} &= \sum_{ k \in \mathbb{N}, k\ {\rm even}}  \frac{1}{144} (k+1)(k+2)(k+3)^2 (k+4)(k+5),\\
			\Sigma_{o} &= \sum_{ k \in \mathbb{N}, k\ {\rm odd}}  \frac{1}{144} (k+1)(k+2)(k+3)^2 (k+4)(k+5),\\
		\end{aligned}
	\end{equation}
	For $k = 1$ and $k = 4$, AdS/CFT dictates:
	\begin{equation}
		\left. \begin{aligned}
			& \Sigma_e + \Sigma_o = \frac{1}{6}, \quad (k = 1),\\
			& \frac{1}{2} \Sigma_e = \frac{1}{6},\quad (k = 4),\\
			% & \frac{1}{3} \Sigma_e = \frac{1}{6},\quad (k = 3).\\
		\end{aligned} \right\}  \Rightarrow \Sigma_e = \frac{1}{3},\quad \Sigma_o = - \frac{1}{6}.
	\end{equation}
	Now let's consider $k = 3$, where AdS/CFT dictates:
	\begin{equation}
		\frac{1}{3} \Sigma_e + (\delta a_E^{k = 3})^{\rm tot} = \frac{1}{6} \quad \Rightarrow \quad  (\delta a_E^{k = 3})^{\rm tot} = \frac{1}{18} \ne 0!
	\end{equation}
	For general $k$, we should have
	\begin{equation}
		\frac{1}{k'} \Sigma_e +  (\delta a_E^{k'})^{\rm tot} = \frac{1}{6} \quad \Rightarrow \quad \boxed{ (\delta a_E^{k'})^{\rm tot}  = \frac{1}{6} - \frac{1}{3k'}} ,
	\end{equation}
	although the Friedman regularisation dictates them to be zero. This is reminiscent of our prescription for $(a_E^{k = 1})^{\rm tot}$ in the original ABJM theory. 

	\subsection{KK supergravity connected to the SO(8) gauged supergravity} \label{app:SO8}
		We present our calculations for the $(a_E, c, b_1)$ coefficients in supergravity theories connected to the SO(8) gauged supergravity by RG flows apart from the one dual to the mABJM theory discussed above. The theories are shown in Fig. \ref{fig:ABJMRGWebs}. 
		
		\subsubsection{Theory 1: $\cN = 1, G_2$}
		We start with the $\cN = 1$ fixed point with $G_2$ flavor group, given by the quadratic deformation of ABJM and is dual to the
		CPW solution \cite{Corrado:2001nv} in 11d supergravity. The supergravity multiplets can be mapped to the 3d $\cN = 1$ superconformal multiplets discussed above Table~\ref{HeatKernelCoefficientsN=1Multiplets}. 
		
		The Kaluza-Klein mass spectrum can be evaluate using the Exceptional Field Theory technique \cite{Cesaro:2020soq}. At level $k = 0$, different from the SO(8) theory, some of the  gaugini and vector fields acquire mass by eating some scalars and fermions. Using the multiplets shown in Table 2 of \cite{Cesaro:2020soq}, we can explicitly check that
		\begin{equation}
		(a_E)_0 = \frac{5}{2},\quad c_0 = (b_1)_0 = 0,
		\end{equation}
		which is consistent with the GR flow conjecture. At level $k\ge 1$, all the multiplets are massive and thus long, since all the short $\cN = 1$ multiplets are massless. Thus, knowing the branching rules from SO(8) to $G_2$ will teach us the full knowledge of the multiplets.
		\begin{equation}
		{\rm Gravitons:}\qquad (k000) \rightarrow \bigoplus_{p = 0}^k (p0)
		\end{equation}
		Each graviton corresponds to a LGRAV(we only consider $k\ge 1$):
		\begin{equation}
		\boxed{ {\rm LGRAV:}\qquad \bigoplus_{p = 0}^k (p0) }
		\end{equation}
		\begin{equation}
		\begin{aligned}
		{\rm Gravitini:}\qquad (k001) &\rightarrow \left[\bigoplus_{p = 0}^{k-1} (p1) \right] \oplus \left[\bigoplus_{p = 0}^{k+1} (p0) \right] \oplus \left[\bigoplus_{p = 1}^{k} (p0) \right] \\
		(k-1,0,1,0) &\rightarrow \left[\bigoplus_{p = 0}^{k-2} (p1) \right] \oplus \left[\bigoplus_{p = 0}^{k} (p0) \right] \oplus \left[\bigoplus_{p = 1}^{k-1} (p0) \right] \\
		\end{aligned}
		\end{equation}
		One LGRAV has two gravitini, and the remaining gravitini correspond to the highest-spin component of LGINOs, which are:
		\begin{equation}
		\boxed{ {\rm LGINO}:\qquad \left[\bigoplus_{p = 0}^{k-1} (p1) \right] \oplus \left[\bigoplus_{p = 0}^{k-2} (p1) \right] \oplus \left[\bigoplus_{p = 1}^{k+1} (p0) \right] \oplus \left[\bigoplus_{p = 1}^{k-1} (p0) \right] }
		\end{equation}
		\begin{equation}
		\begin{aligned}
		{\rm Vectors:}\qquad (k100) &\rightarrow \left[\bigoplus_{p = 0}^{k} (p1) \right] \oplus \left[\bigoplus_{p = 0}^{k-1} (p1) \right] \oplus \left[\bigoplus_{p = 1}^{k+1} (p0) \right]^{\oplus 2}\\
		(k-1,0,1,1) & \rightarrow \left[\bigoplus_{p = 0}^{k-3} (p2) \right] \oplus \left[\bigoplus_{p = 0}^{k-1} (p1) \right] \oplus \left[\bigoplus_{p = 0}^{k-2} (p1) \right]^{\oplus 2} \oplus \left[\bigoplus_{p = 1}^{k-1} (p1) \right] \oplus \\
		& \oplus \left[\bigoplus_{p = 0}^{k+1} (p0) \right] \oplus \left[\bigoplus_{p = 1}^{k} (p0) \right] \oplus \left[\bigoplus_{p = 1}^{k-1} (p0) \right] \oplus \left[\bigoplus_{p = 2}^{k} (p0) \right] \\
		(k-2,1,0,0) &\rightarrow \left[\bigoplus_{p = 0}^{k-2} (p1) \right] \oplus \left[\bigoplus_{p = 0}^{k-3} (p1) \right] \oplus \left[\bigoplus_{p = 1}^{k-1} (p0) \right]^{\oplus 2}\\
		\end{aligned}
		\end{equation}
		For each LGRAV, there is 1 vector field; and for each LGINO, there are 2 vector fields. Each of the remaining vector fields corresponds a LVEC:
		\begin{equation}
		\boxed{ \begin{aligned}
			{\rm LVEC:} \qquad & \left[\bigoplus_{p = 0}^{k-3} (p2) \right] \oplus \left[\bigoplus_{p = 0}^{k} (p1) \right] \oplus \left[\bigoplus_{p = 1}^{k-1} (p1) \right] \oplus \left[\bigoplus_{p = 0}^{k-2} (p1) \right] \oplus \left[\bigoplus_{p = 0}^{k-3} (p1) \right] \oplus\\
			& \oplus \left[\bigoplus_{p = 1}^{k+1} (p0) \right] \oplus \left[\bigoplus_{p = 2}^{k} (p0) \right] \oplus \left[\bigoplus_{p = 1}^{k-1} (p0) \right]  \\
			\end{aligned} }
		\end{equation}
		\begin{equation}
		\begin{aligned}
		{\rm Fermions:}\qquad (k+1,0,1,0) &\rightarrow  \left[\bigoplus_{p = 0}^{k} (p1) \right] \oplus \left[\bigoplus_{p = 0}^{k+2} (p0) \right]  \oplus \left[\bigoplus_{p = 1}^{k+1} (p0) \right]    \\
		(k-1, 1,1,0) & \rightarrow \left[\bigoplus_{p = 0}^{k-2} (p2) \right] \oplus \left[\bigoplus_{p = 0}^{k-3} (p2) \right] \oplus \\
		\oplus \left[\bigoplus_{p = 0}^{k} (p1) \right] & \oplus \left[\bigoplus_{p = 0}^{k-1} (p1) \right] \oplus \left[\bigoplus_{p = 0}^{k-2} (p1) \right] \oplus \left[\bigoplus_{p = 1}^{k-1} (p1) \right]^{\oplus 2} \oplus\\
		& \oplus \left[\bigoplus_{p = 1}^{k+1} (p0) \right]^{\oplus 2}  \oplus \left[\bigoplus_{p = 2}^{k} (p0) \right]^{\oplus 2} \\
		(k-2, 1,0,1) & \rightarrow \left[\bigoplus_{p = 0}^{k-3} (p2) \right] \oplus \left[\bigoplus_{p = 0}^{k-4} (p2) \right] \oplus \\
		\oplus \left[\bigoplus_{p = 0}^{k-1} (p1) \right] & \oplus \left[\bigoplus_{p = 0}^{k-2} (p1) \right] \oplus \left[\bigoplus_{p = 0}^{k-3} (p1) \right] \oplus \left[\bigoplus_{p = 1}^{k-2} (p1) \right]^{\oplus 2} \oplus\\
		& \oplus \left[\bigoplus_{p = 1}^{k} (p0) \right]^{\oplus 2}  \oplus \left[\bigoplus_{p = 2}^{k-1} (p0) \right]^{\oplus 2} \\
		(k-2,0,0,1) &\rightarrow  \left[\bigoplus_{p = 0}^{k-3} (p1) \right] \oplus \left[\bigoplus_{p = 0}^{k-1} (p0) \right]  \oplus \left[\bigoplus_{p = 1}^{k-2} (p0) \right]    \\
		\end{aligned}
		\end{equation}
		For each LGINO, there is 1 vector field; for each LVEC, there are 2 vector fields.
		\begin{equation}
		\boxed{ \begin{aligned}
			{\rm LSCA:} \qquad & \left[\bigoplus_{p = 0}^{k-2} (p2) \right] \oplus \left[\bigoplus_{p = 0}^{k-4} (p2) \right] \oplus  \left[\bigoplus_{p = 1}^{k-1} (p1) \right] \oplus \left[\bigoplus_{p = 1}^{k-2} (p1) \right] \oplus \\
			&  \oplus \left[\bigoplus_{p = 0}^{k+2} (p0) \right]  \oplus \left[\bigoplus_{p = 0}^{k} (p0) \right]  \oplus \left[\bigoplus_{p = 2}^{k} (p0) \right] \oplus \left[\bigoplus_{p = 2}^{k-2} (p0) \right]   \\
			\end{aligned} }
		\end{equation}
		Having obtained all the multiplets, it becomes straightforward to evaluate the heat-kernel coefficients. We can check explicitly that with the $G_2$ matter contents given above that\footnote{In order to evaluate $(b_1)_k$, we need to use $E_0$ for different multiplets given in equation (3.1) of \cite{Cesaro:2020soq}.} $$(a_E)_k = \frac{1}{144}(k+1)(k+2)(k+3)^2 (k+4)(k+5),\quad c_k = (b_1)_k = 0.$$
		
		\subsubsection{Theory 2 and 3: $\cN = 1$ with SO(3) and U(1)$^2$}
		Because of the much smaller flavor symmetries, these two theories are under less analytical control. However, exceptional field theory helps getting the numerical mass spectrum for the low-lying Kaluza-Klein modes. With the numerical data given by \cite{Cesaro:2021haf}, we are able to numerically check that the same values of coefficients are reproduced.\footnote{We thank the authors of \cite{Cesaro:2021haf} for providing the codes of the data and pointing out some typos in the original paper. }
		
	%%%%%%%%%%%%%%%%%%%%%%%%5
	\subsection{KK supergravity connected to the ISO(7) gauged supergravity} \label{app:ISO7}
	Now we proceed to theories connected to the ISO(7) gauged supergravity, which can be uplifted to the massive type IIA supergravity in 10d. There is a slightly more intricated web of flows shown in Fig.~\ref{fig:ISO(7)gaugedSugraRGWebs}, which we expect the heat-kernel coefficients to be identical level-by-level. 
	
	In this example, the ``UV'' theory is given by the maximal ISO(7) gauged supergravity, which can be obtained by compactifying massive type IIA supergravity on $S^6$. The theory is not conformal, but the fields are still organized into KK-levels and transform irreducibly under the SO(7) gauge group.\footnote{See, for example, Table 1 of \cite{Varela:2020wty}. } 
	
	In this part, we will start presenting the five theories with large flavor symmetries in Fig.~\ref{fig:ISO(7)gaugedSugraRGWebs}, i.e. (1) the $\cN = 2, SU(3)\times U(1)$ theory, (2) the $\cN = 1, G_2$ theory, (3) the $\cN = 0, G_2$ theory, (4) the $\cN = 0, SO(7)$ theory, and (5) the $\cN = 0, SO(6)$ theory. Benefiting from the large symmetry group, we can obtain the multiplet contents analytically by branching rules for all KK level. After that, we present two less symmetric theories, they are: (6) the $\cN = 3, SO(4)$ theory and (7) the $\cN = 1, SU(3)$ theory. For these two theories, we are not able to write down all the multiplets analytically, but we can indirectly get the heat-kernel coefficients summed over all fields at a given KK level. Lastly, there are three theories with very small global symmetries, including: (8) the $\cN = 1, U(1)_a$ theory, (9) the $\cN = 1, U(1)_b$ theory and (10) the $\cN = 1, \emptyset$ theory without any global symmetry.\footnote{We add the label $a$ and $b$ only to distinguish the two theories, there is no special meaning to this notation. } For these three theories, there are only numerical spectrum available for the low-lying modes. 
	
	\subsubsection{Theory 1: $\cN = 2, SU(3) \times U(1)$}
		The mass spectrum is given in \cite{Varela:2020wty}. The heat-kernel coefficients for 3d $\cN = 2$ superconformal multiplets are given in Table~\ref{HeatKernelCoefficientsMultiplets}. We start with the long multiplets, which are easier because their contributions to the coefficients are all numbers. So we only need to count the long multiplets, without knowing in details the branching rules from SO(7) to SU(3)$\times$U(1). The procedure will be similar to what we did for mABJM above. 
		
		The SU(3)$\times$U(1) irrep of the LGRAVs are explicitly known in \cite{Varela:2020wty}:
		\begin{equation}
		\bigoplus_{l=0}^{k-1} \bigoplus_{p=0}^l[p, l-p]_{\frac{2}{3}(l-2p)} \oplus \bigoplus_{p=1}^{k-1} [p, k-p]_{\frac{2}{3}(k-2p)},
		\end{equation}
		the dimension for which is\footnote{Notice that when $k = 0$, the sum over $p$ from $1$ to $k$ generates an undesired term, so we added $\delta_{k,0}$ to cancel it. }
		\begin{equation}
		\boxed{ \Omega_{k}^{\rm LGRAV} = \frac{1}{120}(k+1)(k+2)(2k^3 + 19k^2 + 59k - 60) + \delta_{k,0}. }
		\end{equation}
		The number of LGINO is given by:
		\begin{equation*}
		\begin{aligned}
		\Omega_k^{\rm LGINO} &= \dim[k,0,1] + \dim[k-1,0,1] - 4 \Omega_k^{\rm LGRAV} - 3 \Omega_k^{\rm SGRAV} - 2 \Omega_k^{\rm MGRAV} -  \Omega_k^{\rm SGINO} \\
		\end{aligned}
		\end{equation*}
		\begin{equation}
		\Rightarrow \quad  \boxed{ \Omega_k^{\rm LGINO} = \frac{1}{30} k(k+1)(k+4)(2k^2 + 15k + 37). }
		\end{equation}
		In the same way, the number of LVEC is\footnote{We introduce the delta on the first line to solve the problem $\dim [k-2,1,0] \ne 0$ for $k = 0$. }
		\begin{equation*}
		\begin{aligned}
		\Omega_k^{\rm LVEC} &= \frac{9}{40}(k+1)(k+2)(k+3)(k+4)(2k+5) + \delta_{k,0}\\
		& - 6 \Omega_k^{\rm LGRAV} - 3 \Omega_k^{\rm SGRAV} - \Omega_k^{\rm LGRAV} - 4 \Omega_k^{\rm LGINO} - 3 \Omega_k^{\rm SGINO} - \Omega_k^{\rm SVEC} - \Omega_k^{\rm MVEC}
		\end{aligned}
		\end{equation*}
		\begin{equation}
		\Rightarrow \quad  \boxed{ \Omega_k^{\rm LVEC} = \frac{1}{24}(k+3)(k+4)(2k^3 + 11k^2 + 19k - 14) + 8 \delta_{k,0}. }
		\end{equation}
		
		Now we turn to the short multiplets. From Table~\ref{HeatKernelCoefficientsMultiplets}, we realize that $a_E$ and $c$ doesn't depend on the conformal dimension of the superconformal primaries, so the total coefficient is given by the coefficient for a single multiplet times their numbers $\Omega_k^{X}$, where $X$ denotes a multiplet:
		\begin{equation}
		\begin{aligned}
		\Omega_k^{\rm SGRAV} &= (k+1)(k+2) - 2\delta_{k,0},\quad  \Omega_k^{\rm MGRAV} = \delta_{k,0},\\
		\Omega_k^{\rm SGINO} &= 2(k+1)(k+3),\\
		\Omega_k^{\rm S/MVEC} &=2(k+2)(k+4) - 16\delta_{k,0},\quad \Omega_k^{\rm MVEC} = 8 \delta_{k,0},\\
		\Omega_k^{\rm HYP} &= (k+3)(k+4).\\
		\end{aligned}
		\end{equation}
		However, $b_1$ does depends on the conformal dimension of the superconformal primaries, so we need to do calculate independently:
		\begin{equation}
		\begin{aligned}
		(b_1)_k^{\rm SGRAV} &= -\frac{1}{432}(k+1)(k+2)(4k^2+36k-27)-\frac{1}{8}\delta_{k,0},\\
		(b_1)_k^{\rm SGINO} &= \frac{1}{216}(k+1)(k+3) (4k^2+28k-5),\\
		(b_1)_k^{\rm SVEC} &= - \frac{1}{216} (k+2)(k+4)(4k^2+12k-9) - \frac{1}{3} \delta_{k,0} ,\\
		(b_1)_k^{\rm HYP} &= \frac{1}{432}(k+3)(k+4)(2k+1)^2.\\
		\end{aligned}
		\end{equation}
		At the lowest KK-level, multiplets can be massless, which contribute:
		\begin{equation}
		(b_1)_k^{\rm MGRAV} = 0,\quad (b_1)_k^{\rm MVEC} = 0.
		\end{equation}
		Summing over all the multiplets, we get:
		\begin{equation} \label{eq:HKmIIA}
		\boxed{ \begin{aligned}
		(a_E)_k &= \frac{1}{48} (k+1)(k+2)(k+3)(k+4)(2k+5),\\
		c_k &= (b_1)_k = 0.
		\end{aligned} }
		\end{equation}
		This is a new prediction. To support the Conjecture \ref{LogNRGFlowConjecture}, one should show in all the other theories in Fig.~\ref{fig:ISO(7)gaugedSugraRGWebs} give the same results level-by-level.
		
		\subsubsection{Theory 2 and 3: $\cN = 1, G_2$ and $\cN = 0, G_2$ }
		Let's start with the $G_2$ theory with $\cN = 1$. The spectrum of this theory is discussed in \cite{Cesaro:2020soq}. For $\cN = 1$ multiplets, the heat-kernel coefficients do depend on the masses, so we need to honestly use the branching rules to get all the multiplets, which is possible thanks to the large global $G_2$ symmetry.\footnote{Notice that the contents we get below doesn't seem to correctly reproduce the coefficients for $k = 2$, which is likely a mistake of mine. But luckily it is only for $k = 2$, where the branching can be done seperatedly, and I checked that it is fine.} 
		\begin{equation}
		\boxed{ {\rm LGRAV:} [k,0,0]\rightarrow [k,0]. }
		\end{equation}
		\begin{equation}
		\begin{aligned}
		{\rm Gravitini:} [k,0,1]&\rightarrow [k,0] \oplus [k+1,0] \oplus [k-1,1],\\
		[k-1,0,1]& \rightarrow [k-1,0] \oplus [k,0]_{k \ge 1} \oplus [k-2,1].\\
		\end{aligned}
		\end{equation}
		\begin{equation}
		\Rightarrow\quad  \boxed{ {\rm LGINO:}\  [k+1,0] \oplus [k-1,0] \oplus [k-1,1] \oplus [k-2,1]. }
		\end{equation}
		\begin{equation}
		\begin{aligned}
		{\rm Vectors:} [k,1,0]&\rightarrow [k+1,0] \oplus [k,1] \oplus [k-1,1],\\
		[k-1,1,0]&\rightarrow [k,0]_{k \ge 1} \oplus [k-1,1] \oplus [k-2,1],\\
		[k-2,1,0]&\rightarrow [k-1,0]_{k \ge 2} \oplus [k-2,1] \oplus [k-3,1],\\
		[k-1,0,2]& \rightarrow [k-1,0] \oplus [k,0]_{k \ge 1} \oplus [k+1,0]_{k \ge 1} \oplus [k-2,1] \oplus \\
		& \qquad  \oplus [k-1,1]_{k\ge 2} \oplus [k-3,2],\\
		[k+1,0,0]&\rightarrow [k+1,0],\\ 
		[k-1,0,0]&\rightarrow [k-1,0].\\ 
		\end{aligned}
		\end{equation}
		\begin{equation}
		\boxed{
			\begin{aligned}
			{\rm LVEC:}\ & [k+1,0]_{k \ge 1} \oplus [k,0]_{k \ge 1} \oplus [k-1,0]_{k \ge 2} \oplus \\
			& \oplus [k,1] \oplus [k-1,1]_{k\ge 2} \oplus [k-2,1]  \oplus [k-3,1] \oplus [k-3,2].
			\end{aligned}
		}
		\end{equation}  
		\begin{equation}
		\begin{aligned}
		{\rm Spinors:}\ [k+1,0,1]\rightarrow& [k+1,0] \oplus [k+2,0] \oplus [k,1],\\
		[k,0,1] &\rightarrow [k,0] \oplus [k+1,0] \oplus [k-1,1],\\
		[k-1,0,1]& \rightarrow [k-1,0] \oplus [k,0]_{k \ge 1} \oplus [k-2,1],\\
		[k-2,0,1]& \rightarrow [k-2,0] \oplus [k-1,0]_{k \ge 2} \oplus [k-3,1],\\
		[k-1,1,1]\rightarrow & [k,0]_{k\ge 1} \oplus [k+1,0]_{k\ge 1} \oplus [k-1,1] \oplus [k,1]_{k\ge 1} \oplus \\
		& \oplus  [k-2,1] \oplus [k-1,1]_{k\ge 2} \oplus [k-2,2] \oplus [k-3,2],\\
		[k-2,1,1]\rightarrow & [k-1,0]_{k\ge 2} \oplus [k,0]_{k\ge 2} \oplus [k-2,1] \oplus [k-1,1]_{k\ge 2} \oplus \\
		& \oplus  [k-3,1] \oplus [k-2,1]_{k\ge 3} \oplus [k-3,2] \oplus [k-4,2].\\
		\end{aligned} 
		\end{equation}
		\begin{equation}
		\boxed{ \begin{aligned}
			{\rm LSCA:} & \ [k+2,0] \oplus [k,0] \oplus [k,0]_{k\ge 2} \oplus [k-2,0] \oplus [k-1,1] \oplus [k-2,1] \oplus \\
			&\qquad  \oplus [k-2,2] \oplus [k-4,2].
			\end{aligned} }
		\end{equation}
		With the explicit multiplets contents together with the spctrum given in \cite{Cesaro:2020soq}, we can reproduce the contributions in \eqref{eq:HKmIIA}.
		
		For the $G_2$ theory with $\cN = 0$, there is no multiplet structures and all fields are standing on their own. Their transform irreducibly under the flavor group with representations given by the branching rules above. In addition, the scalars transform under:
		\begin{equation}
		\begin{aligned}
		{\rm Scalars:} [k+2,0,0] &\rightarrow [k+2,0],\\
		[k,0,0] & \rightarrow [k,0],\\
		[k-2,2,0] &\rightarrow [k,0]_{k\ge 2} \oplus [k-1,1]_{k\ge 2} \oplus [k-2,2] \oplus [k-3,2] \oplus \\
		& \oplus [k-2,1]_{k\ge 3} \oplus [k-4,2], \\
		[k-2,0,0] &\rightarrow [k-2,0],\\
		[k,0,2]& \rightarrow [k,0] \oplus [k+1,0] \oplus [k+2,0] \oplus [k-1,1] \oplus [k,1]_{k\ge 1} \oplus [k-2,2],\\
		[k-1,1,0]&\rightarrow [k,0]_{k \ge 1} \oplus [k-1,1] \oplus [k-2,1],\\
		[k-2,0,2]& \rightarrow [k-2,0] \oplus [k-1,0]_{k \ge 2} \oplus [k,0]_{k \ge 2} \oplus [k-3,1] \oplus \\
		& \oplus [k-2,1]_{k\ge 3} \oplus [k-4,2].\\
		\end{aligned}
		\end{equation}
		The representations for fields with spins ranging from 0 to 2, together with the mass spectra of the $\cN=0, G_2$ given in \cite{Cesaro:2020soq}, is enough for us to check that the coefficients are indeed identical to \eqref{eq:HKmIIA}.
		
		\subsubsection{Theory 4 and 5: $\cN = 0, SO(7)$ and $\cN = 0, SO(6)$}
		We start with the SO(7) theory with larger symmetry. The multiplets are given in Table 1 of \cite{Varela:2020wty}. There is one subtlety at $k = 0$ level, where the gravitini are massive and eat 8 spinors under the same representation. The vectors in $\bf 7$ of SO(7) are also massive, whose scalar Stuckelburg fields are already excluded from the table. So the correct field contents at $k = 0$ are given in Table \ref{k=0N0SO7mIIA}.
		\begin{table}[!h]
			\renewcommand{\arraystretch}{1.8}
			\centering
			\begin{tabular}{c|c|c}
				\hline 
				spin  & SO(7) representation & $ml$ \\ \hline 
				2 & (000) & 0\\
				$\frac{3}{2}$ &  (001) & $ \frac{3\sqrt{15}}{10} $\\
				1 & (010) $\oplus $ (100) & $0, \ \ 2\sqrt{\frac{3}{5}} $ \\
				$\frac{1}{2}$ & (101)  & $\frac{\sqrt{15}}{10} $\\
				$0_+$ & (200)$  \oplus$(000)  & $2\sqrt{-\frac{3}{5} },\ \  \sqrt{6} $\\
				$0_-$ & (002) & $ \sqrt{-\frac{6}{5}}$\\
			\end{tabular}
			\caption{\rm Fields in the $k = 0$ level of the $\cN = 0$ SO(7) theory.}
			\label{k=0N0SO7mIIA}
		\end{table}
	
		Using the mass spectra given in \cite{Varela:2020wty}, we can reproduce \eqref{eq:HKmIIA} for both $k=0$ and larger $k\ge 1$.
		
		For the $\cN = 0$ SO(6) theory, the fields are organized into the representations of SO(6)$\sim$SU(4) under the branching of SO(7):
		\begin{equation}
		\begin{aligned}
		{\rm Gravitons:}\qquad (k00) &\rightarrow \bigoplus_{p=0}^k (0p0). \\
		\end{aligned}
		\end{equation}
		\begin{equation}
		\begin{aligned}
		{\rm Gravitini:}\qquad (k01) &\rightarrow \left[\bigoplus_{p=0}^{k} (1p0) \right] \oplus \left[\bigoplus_{p=0}^{k} (0p1) \right], \\
		(k-1,0,1) &\rightarrow \left[\bigoplus_{p=0}^{k-1} (1p0) \right] \oplus \left[\bigoplus_{p=0}^{k-1} (0p1) \right], \\
		\end{aligned}
		\end{equation}
		\begin{equation}
		\begin{aligned}
		{\rm Vectors:}\qquad (k-1,0,2) &\rightarrow \left[\bigoplus_{p=0}^{k-1} (1p1) \right] \oplus \left[\bigoplus_{p=0}^{k-1} (2p0) \right] \oplus \left[\bigoplus_{p=0}^{k-1} (0p2) \right] , \\
		(k10) &\rightarrow \left[\bigoplus_{p=1}^{k+1} (0p0) \right] \oplus \left[\bigoplus_{p=0}^{k} (1p1) \right], \\
		(k-1,1,0) &\rightarrow \left[\bigoplus_{p=1}^{k} (0p0) \right] \oplus \left[\bigoplus_{p=0}^{k-1} (1p1) \right], \\
		(k-2,1,0) &\rightarrow \left[\bigoplus_{p=1}^{k-1} (0p0) \right] \oplus \left[\bigoplus_{p=0}^{k-2} (1p1) \right], \\
		(k+1,0,0) &\rightarrow \bigoplus_{p=0}^{k+1} (0p0), \\
		(k-1,0,0) &\rightarrow \bigoplus_{p=0}^{k-1} (0p0), \\
		\end{aligned}
		\end{equation}
		\begin{equation}
		\begin{aligned}
		{\rm Spinors:}\qquad (k+1,0,1) &\rightarrow \left[\bigoplus_{p=0}^{k+1} (1p0) \right] \oplus \left[\bigoplus_{p=0}^{k+1} (0p1) \right], \\
		(k,0,1) &\rightarrow \left[\bigoplus_{p=0}^{k} (1p0) \right] \oplus \left[\bigoplus_{p=0}^{k} (0p1) \right], \\
		(k-1,0,1) &\rightarrow \left[\bigoplus_{p=0}^{k-1} (1p0) \right] \oplus \left[\bigoplus_{p=0}^{k-1} (0p1) \right], \\
		(k-2,0,1) &\rightarrow \left[\bigoplus_{p=0}^{k-2} (1p0) \right] \oplus \left[\bigoplus_{p=0}^{k-2} (0p1) \right], \\
		(k-1,1,1) &\rightarrow \left[\bigoplus_{p=1}^{k} (1p0) \right] \oplus \left[\bigoplus_{p=0}^{k-1} (2p1) \right] \oplus \left[\bigoplus_{p=1}^{k} (0p1) \right] \oplus \left[\bigoplus_{p=0}^{k-1} (1p2) \right],  \\
		(k-2,1,1) &\rightarrow \left[\bigoplus_{p=1}^{k-1} (1p0) \right] \oplus \left[\bigoplus_{p=0}^{k-2} (2p1) \right] \oplus \left[\bigoplus_{p=1}^{k-1} (0p1) \right] \oplus \left[\bigoplus_{p=0}^{k-2} (1p2) \right],  \\
		\end{aligned}
		\end{equation}
		\begin{equation}
		\begin{aligned}
		{\rm Scalars_+:}\qquad (k+2,0,0) &\rightarrow \bigoplus_{p=0}^{k+2} (0p0), \\
		(k,0,0) &\rightarrow \bigoplus_{p=0}^{k} (0p0), \\
		(k-2,0,0) &\rightarrow \bigoplus_{p=0}^{k-2} (0p0), \\
		(k-2,2,0) & \rightarrow \left[ \bigoplus_{p=2}^k (0p0) \right] \oplus \left[ \bigoplus_{p=1}^{k-1} (1p1) \right] \oplus \left[ \bigoplus_{p=0}^{k-2} (2p2) \right] 
		\end{aligned}
		\end{equation}
		\begin{equation}
		\begin{aligned}
		{\rm Scalars_-:}\qquad (k,0,2) &\rightarrow \left[\bigoplus_{p=0}^{k} (1p1) \right] \oplus \left[\bigoplus_{p=0}^{k} (2p0) \right] \oplus \left[\bigoplus_{p=0}^{k} (0p2) \right] , \\
		(k-2,0,2) &\rightarrow \left[\bigoplus_{p=0}^{k-2} (1p1) \right] \oplus \left[\bigoplus_{p=0}^{k-2} (2p0) \right] \oplus \left[\bigoplus_{p=0}^{k-2} (0p2) \right] , \\
		(k-1,1,0) &\rightarrow \left[\bigoplus_{p=1}^{k} (0p0) \right] \oplus \left[\bigoplus_{p=0}^{k-1} (1p1) \right]. \\
		\end{aligned}
		\end{equation}
		Again, one has to be careful for $k = 0$, where we have collected the correct field contents in Table \ref{k=0N0SU(4)mIIA}. Compared to the SO(7) theory, the vectors in $(010)$ of SO(7) become massive, which eat scalars in the $(010)\oplus(101)$ of SU(4). With the the mass formulas given in Table 17 of \cite{Cesaro:2020soq}, we can reproduce \eqref{eq:HKmIIA} for $k = 0$ and $k\ge 1$.
		\begin{table}[!h]
			\renewcommand{\arraystretch}{1.8}
			\centering
			\begin{tabular}{c|c|c}
				\hline 
				spin  & SU(4) irrep & $ml$ \\ \hline 
				2 & (000) & 0\\
				$\frac{3}{2}$ & (100) $\oplus $ (001) & $\frac{3}{2}, \frac{3}{2}$\\
				1 & (000) $\oplus $ (010)$^2\oplus$(101) & $\sqrt{6}, \sqrt{3}, \sqrt{\frac{6}{5}}$ \\
				$\frac{1}{2}$ & (001)$\oplus$(011)$\oplus$(100)$\oplus$(110) & $\frac{\sqrt{21}}{2}, \frac{\sqrt{165}}{10}, \frac{\sqrt{21}}{2}, \frac{\sqrt{165}}{10} $\\
				$0_+$ & (000)$^2 \oplus$ (020) & $\sqrt{6}, \sqrt{-\frac{6}{5}}$\\
				$0_-$ & (200) $\oplus$ (002) & $\sqrt{\frac{3}{5}}, \sqrt{\frac{3}{5}}$\\
			\end{tabular}
			\caption{\rm Fields in the $k = 0$ level of the $\cN = 0$ SU(4) theory from mIIA supergravity.}
			\label{k=0N0SU(4)mIIA}
		\end{table}
		
		\subsubsection{Theory 6 and 7: $\cN = 3, SO(4)$ and $\cN = 1, SU(3)$}
		We put together these two theories because we are able to evaluate the coefficients $(a_E, c, b_1)$ for a given KK level, but we are not able to get the multiplet contents explicitly in a closed form. Nevertheless, this is enough for supporting our conjecture \ref{LogNRGFlowConjecture}.
		
		We start with the $\cN = 3, SO(4)$ theory, which is connected to the $\cN = 2, SU(3)\times U(1)$ theory and the $\cN = 1, G_2$ theory by holographic RG flows as shown in Fig.\ref{fig:ISO(7)gaugedSugraRGWebs} reviewed in \cite{Guarino:2019snw}. According to the coefficients of $\cN = 3$ multiplets evaluated in \eqref{eq:HKEN3Multiplets}, $b_1$ vanishes for all the multiplets and $c$ vanishes for all the long multiplets. We shall start with the short multiplets whose contents are known explicitly for any KK level \cite{Varela:2020wty}, as shown in Table \ref{table:ShortMultipletsSO4IIA}. The multiplets transform irreducibly under the global symmetry $SO(4) = SO(3)_F \times SO(3)_R$.
		\begin{table}[!h]
			\renewcommand{\arraystretch}{1.5}
			\centering
			\begin{tabular}{ccc}
				multiplet & SO(3)$_F\times$SO(3)$_R$ & $E_0$ \\ \hline 
				SGRAV$_3$ & $(0,k)$ & $k+\frac{3}{2}$ \\
				SGINO$_3$ & $\left( \frac{k+1}{2}, \frac{k+1}{2} \right)$ & $\frac{k+3}{2}$ \\
				SVEC$_3$ & $\left( \frac{k+2}{2}, \frac{k+2}{2} \right)$ & $\frac{k+2}{2}$ \\ \hline 
			\end{tabular}
			\caption{\rm All the short $\cN = 3$ multiplets in SO(4) theory. Copied from Table 8 of \cite{Varela:2020wty}. $k$ is the KK-level.}
			\label{table:ShortMultipletsSO4IIA}
		\end{table}
	With the coefficients given in \eqref{eq:HKEN3Multiplets}, we directly get:
	\begin{equation*}
	\begin{aligned}
	(a_E)_k^{\rm short} &= \dim\left[ 0 \right] (a_E)_k^{\rm SGRAV_3} + \dim\left[ \frac{k+1}{2} \right] (a_E)_k^{\rm SGINO_3} + \dim\left[ \frac{k+2}{2} \right] (a_E)_k^{\rm SVEC_3}\\
	&  = \frac{1}{2}(k^2+8k+4),\\
	c_k &= \dim\left[ 0 \right] c_k^{\rm SGRAV_3} + \dim\left[ \frac{k+1}{2} \right] c_k^{\rm SGINO_3} + \dim\left[ \frac{k+2}{2} \right] c_k^{\rm SVEC_3} = 0,\\
	\end{aligned}
	\end{equation*}
	The result for $c_k$ is consistent with our conjecture \ref{LogNRGFlowConjecture}. We need to proceed to the long multiplets for $a_E$. Since $a_E$ depends on the $R$-charges, we need the representations of all the long multiplets apart from their numbers, which requires us to do the following branching:
	\begin{equation} \label{BranchingSO7toSO4}
	{\rm SO(7)} \supset {\rm SO(3)}_F \times [{\rm SO(3)}\times {\rm SO(3)}] \supset {\rm SO(3)}_F \times {\rm SO(3)}_R,
	\end{equation}
	where SO(3)$_R$ is the diagonal subgroup of $SO(3) \times SO(3)$, whose branching rule is simply:
	\begin{equation}
	[j_1,j_2]\rightarrow [j_1+j_2] \oplus [j_1+j_2-1] \oplus \cdots \oplus [|j_1 - j_2|].
	\end{equation}
	However, it is exactly the appearance of the absolute value that makes the analytic calculation complicated: there are so many different possibilities for the relative signs. So instead of doing the time-consuming brute-force calculation, we do what follows. First, from the branchings together with the expressions of $a_E$ in \eqref{eq:HKEN3Multiplets}, it's not hard to see that $(a_E)_k$ is a polynomial in $k$ of order 5, which can be determined by the six coefficients. To determine them, we explicitly evaluate the irreducible representations of the matter multiplets under $SO(3)_F\times SO(3)_R$ for $k = 0,1,\cdots, 5$. The explicit steps of branching are the same as many other cases we have done, a quick summary:
	\begin{itemize}
		\item $(h, j)$ of LGRAV is obtained by the representations of gravitons, with those in SGRAV substracted.
		\item $(h,j)$ of LGINO is obtained by the representations of gravitini substracting those in SGRAV, LGRAV, and SGINO.
		\item Add up $(a_E)_k^{\rm long}$ with $(a_E)_k^{\rm short}$ obtained above.
	\end{itemize}
	We have checked explicitly for $k = 0,1,\cdots, 13$ that the expression for $(a_E)_k$ is identical to \eqref{eq:HKmIIA} and thus consistent with our conjecture.
	
	For the $\cN = 1, SU(3)$ theory which is the IR fixed point from the $\cN = 1, G_2$ theory, the spectrum is reported in \cite{Cesaro:2020soq}. The group theory exercise we need to work on is:
	\begin{equation}
	SO(7)\rightarrow G_2 \rightarrow SU(3).
	\end{equation}
	Similarly, doing the branchings is possible but complicated, so we used the fact that the heat-kernel coefficients are polynomials of $k$ and evaluated them explicitly for low-lying values of $k$. After working out $k = 0,1,\cdots, 9$, we can confirm the coefficients $(a_E)_k$, $c_k$, and $(b_1)_k$ are identical to \eqref{eq:HKmIIA}.
	
	\subsubsection{Theory 8, 9, and 10: $\cN = 1$, U(1)$_a$, $\cN = 1$, U(1)$_b$, and $\cN = 1$, $\emptyset$}
	Similar to the other theories discussed in \cite{Cesaro:2021haf}, the three theories have very small flavor symmetries, the mass spectra are only known numerically for $k = 0,1,\cdots, 3$. With the available data and mass spactra, we are able to numerically reproduce \eqref{eq:HKmIIA}.
	
	\subsection{Universal conjecture for $c_{\log}$ in TTI }
	Let us recall that $C$ denotes the coefficient of $\log \frac{L}{\sqrt{G}}$ and $\cC$ denotes the coefficient of $\log N$. Because $(b_1)^{\rm tot} = c^{\rm tot} = 0$, we have: 
	\begin{equation}
		C_{\rm nzm}(\cM) = - 2 a_E^{\rm tot} \chi(\cM)
	\end{equation}

	To match with the field theory results, we should consider the 't Hooft limit where $\lambda \equiv N/k$ is fixed. \footnote{ The holographic dictionary is
		\begin{equation}
			e^{\Phi_0} \sim k^{-5/6} N^{-1/6},\quad \frac{\alpha'}{\ell_{s}^2}   \sim \lambda^{-1/3}.
		\end{equation}
		In the 't Hooft limit, the string coupling is zero, and the string tension remains finite.
	} The reason to make this choice is that there are two scaling quantities of the theory:
	\begin{equation}
		\frac{L_{\rm AdS}^2}{G_N } = N^2 \lambda^{-1/3},\qquad \frac{L_{\rm AdS}}{\ell_s} = \lambda^{1/6}.
	\end{equation}
	Thus to get the correct $\log N$ coefficient, one should fix $\lambda$ and assume $\ell_s \gg G_N^{1/2}$, otherwise there will be string modes joining the 1-loop correction.\footnote{This requires $N \gg \lambda^{1/3}$, looser than keeping $\lambda$ fixed. } In the fixed-$\lambda$ limit, we have: \cite{Liu:2018bac,Liu:2019tuk}  
	\begin{equation}
		\begin{aligned}
			& \log Z_{\rm TTI} \supset - \frac{7}{18}(1-\fg) \log N + \frac{1}{18}(1-\fg) \log k = - \frac{1}{3}(1-\fg) \log N - \frac{1}{18} (1-\fg) \log \lambda,\\ 
			& \log Z_{S^3} \supset - \frac{2}{9} \log N + \frac{1}{18} \log k = - \frac{1}{6} \log N - \frac{1}{18} \log \lambda.\\
		\end{aligned}
	\end{equation}
	This perfectly matches the prescription proposed above and imposes:
	\begin{equation}
		a_E^{\rm tot} = \frac{1}{3},\qquad \sum_{k=0}^\infty (k+1)(k+2)(k+3)(k+4)(2k+5) = 16.
	\end{equation}
	Note that the coefficients of $\log \lambda$ are not proportional to the Euler number. This means any non-trivial scaling of $\lambda$ with $N$ will break the proportionality. Now we propose the log coefficient for a IIA SO(7) KK sugra on a general background $\cM$:
	\begin{equation}
		\boxed{ \cC(\cM) = - \frac{1}{6} \chi(\cM). }
	\end{equation}
	For SCI, we expect
	\begin{equation}
		\cC({\rm SCI}) = - \frac{1}{3}.
	\end{equation}
	Similar to the M2-brane theories, here our prescription is exactly consistent with holography. 
	
	%%%%%%%%%%%%%%%%%%%%%%%%%%%%%%%
	%%%%%%%%%%%%%%%%%%%%%%%%%%%%%%%
	\subsection{Theories descending from type IIB supergravity} \label{app:IIB}
	\subsubsection{Theory 1: $\cN = 4\ J_n$ theory}
	In this section, we study theories related to the J-fold theory in type IIB supergravity, whose 10d geometry looks like AdS$_4\times S^1 \times S^5$, where we impose a special twisted boundary condition on $S^1$. The field theory dual is 3d superconformal $J_n$ theory, where the logarithmic term in the partition function vanishes, $c_{\rm log} = 0$ \cite{Assel:2018vtq}, which we would like to reproduce from the gauged supergravity side.
	
	Because of the product form of the internal manifold, we have two sets of KK levels associated to $S^5$ and $S^1$, whose values are $l = 0,1,2,\cdots$, and $n = 0, \pm 1, \pm 2, \cdots$, respectively. The $\cN = 4$ multiplets of the so-called $J_n$ theory are given in \cite{Cesaro:2021tna}, consisting of only graviton multiplets parametrized $[E_0, l_1, l_2]$, where $E_0$ is the dimension of the conformal primary and $(l_1, l_2)$ is the SO(4) $R$-charge. The values of $(l_1, l_2)$ come from the branching $SO(6) \rightarrow SO(4)$:
	\begin{equation}
	[0,l,0]\rightarrow \bigoplus_{a = 0}^{[l/2]} \bigoplus_{k = 0}^{l-2a} [l-2a-k, k].
	\end{equation}
	The dimension of the superconformal primary is given by
	\begin{equation}
	E_0 = -\frac{1}{2} + \sqrt{ \frac{9}{4} + \frac{1}{2}l(l+4) + l_1(l_1+1) + l_2(l_2+1) + \frac{1}{2}\left(\frac{2\pi n}{T} \right)^2 }.
	\end{equation}
	
	Special attention needs to be paid for $m=0, m=1$: for $m = 0$, the multiplet is massless; and for $m = 1$, a few fields are vanishing.\footnote{ Notice that SGRAV[1,0,0] is the stress-momentum multiplet, for which we shouldn't use the table on P.74 of \cite{Cordova:2016emh} but (5.55) in it. } In these cases, the standard Racah-Speiser (RS) algorithm is as follows: \footnote{Introduced in App. B of \cite{Dolan:2002zh} and App. A.3 of \cite{Cordova:2016emh}. }
	\begin{itemize}
		\item If an $R$-charge component of the field is $l = - \frac{1}{2}$, delete it.
		
		\item If an $R$-charge component of the field is $l \le -1$, eat another field with $l = |l| - 1$. The existence of such a field can be proven.
	\end{itemize}
	
	The original field contents in the long and short multiplets can be found in the standard literature \cite{Cordova:2016emh}. With modifications for cases where the $R$-charge has negative components,\footnote{The LGRAV field contents are also given in tables in the App. of \cite{Cesaro:2021tna}, but they contain typos with the special values of the representations. One needs to start with the general field contents and use the RS algorithm to take of the shortening conditions. } we obtain Table \ref{JnLong}.
	
	\begin{table}[h]
		\renewcommand{\arraystretch}{1.5}
		\centering
		\begin{tabular}{c|c|c|c}
			& $a_E$ & $c$ & $b_1$  \\\hline 
			LGRAV$[E_0,0,0]$ & $\frac{5}{2}$ & $0$ & $0$\\
			LGRAV$[E_0,1,0]$ & $\frac{15}{2} $ & $0$ & $0$\\
			LGRAV$[E_0,1,1]$ & $\frac{45}{2}$ & $0$ & $0$\\
			LGRAV$[E_0,l_1,0]$ & $\frac{5}{2}(2l_1+1)$ & $0$ & $0$\\
			LGRAV$[E_0,l_1,1]$ & $\frac{15}{2}(2l_1+1)$ & $0 $ & $0$\\
			LGRAV$[E_0,l_1,l_2]$ & $\frac{5}{2}(2l_1+1)(2l_2+1)$ & $0$ & $0$\\ \hline 
			SGRAV$[2m+1,m,m]$ & $ (4m+1)(2m+1) $ & $  \frac{1}{2}$ & $ 0$\\
			SGRAV$[3,1,1]$ & $ 15 $ & $ \frac{1}{2} $ & $ 0 $\\
			MGRAV$[1,0,0]$ & $1$ & $\frac{1}{2}$ & $ 0$\\ \hline 
			SGINO$[2m+3,m+1,m+1]$ & $ \frac{1}{2}(2m+1)(2m+3) $ & $- \frac{1}{2}$ & $0$ \\
			SGINO$[3,1,1]$ & $ \frac{3}{2} $ & $ -\frac{1}{2} $ & $ 0 $ \\
		\end{tabular}
		\caption{\rm The heat kernel coefficients for 4d $\cN = 4$ LGRAV and SGRAV multiplets. $l_1, l_2 \ge \frac{3}{2}$, $m \ge 2$ in SGRAV and $m\ge 1$ in SGINO.}
		\label{JnLong}
	\end{table}
	
	The unitary bound $E_0 \ge s_0 + l_1 + l_2 + 1$ tells us the values of the charges for which the multiplet shortens:
	\begin{equation}
	n = 0,\quad l_1 = l_2 = \frac{l}{2} = 0,1,2,\cdots,
	\end{equation}
	when the multiplet becomes:
	\begin{equation}
	{\rm LGRAV}_4[l_1+l_2+1,l_1,l_2] \rightarrow {\rm SGRAV}_4[l_1+l_2+1,l_1,l_2] + {\rm SGINO}_4[l_1+l_2+3,l_1+1,l_2+1].
	\end{equation}
	Under the shortening condition, we are interested in SGRAV$[2m+1,m,m]$ and SGINO$[2m+3,m+1,m+1]$ multiplets of 4d $\cN = 4$ sugra, which correspond to $A_2[0]_{\Delta = 2m+1}^{(R=R'=2m)}$ and $B_1[0]_{\Delta=2m+3}^{(R=R'=2m+2)}$ in the notation of \cite{Cordova:2016emh}. 
	
	
	{\bf Case 1: $l = 2m+1, m = 0,1,2,\cdots$}
	
	In this case, there will be no short multiplets. The irreps of SO(4)$_R$ include:
	\begin{equation}
	\begin{aligned}
	[0,2m+1,0] &\rightarrow \bigoplus_{a=0}^{m}\bigoplus_{k=0}^{2(m-a)+1}[2(m-a)+1-k,k] \\
	\end{aligned}
	\end{equation}
	We see that $c_{m,n} = (b_1)_{m,n} = 0$ level-by-level. Though $a_E$ doesn't vanish level-by-level:
	\begin{equation}
	(a_E)_{m,n} = \frac{5}{6}(m+1)(2m+3)^2(m+2) = \frac{5}{24}(l+1)(l+2)^2(l+3),
	\end{equation}
	but we see that $(a_E^{\rm L, odd})_m = 0$ since the summation of $n$ is factored out and $\sum_{n\in \mathbb{Z}} 1 = 0$.
	
	{\bf Case 2: $l = 2m, m = 0,1,2,\cdots$}
	The irreps of SO(4)$_R$ include:
	\begin{equation}
	\begin{aligned}
	[0,2m,0] &\rightarrow \bigoplus_{a=0}^{m}\bigoplus_{k=0}^{2(m-a)}[2(m-a)-k,k] \\
	=& \bigoplus_{p = 0}^m [p,p] \oplus \bigoplus_{a=0}^{m}\bigoplus_{k=0}^{m-a-1}[2(m-a)-k,k] \oplus \bigoplus_{a=0}^{m}\bigoplus_{k=m-a+1}^{2(m-a)}[2(m-a)-k,k].
	\end{aligned}
	\end{equation}
	In this case, we still have $(b_1)_{m,n} = c_{m,n} = 0$ level-by-level. For $(a_E)_m$, the contribution of the last two factors is:
	\begin{equation}
	\frac{5}{6}m(m+1)(2m+1)(2m+3).
	\end{equation}
	Notice that for short multiplets, the contribution to $(a_E)_m$ can be decomposed: ${\rm SGRAV}[2m+1,m,m]+{\rm SGINO}[2m+3,m+1,m+1] = {\rm LGRAV}[E_0,m,m]$, so the total contribution of the first term is:
	\begin{equation}
	\begin{aligned}
	& (1-\delta_{n,0}) \sum_{p = 0}^m \frac{5}{2}(2p+1)^2 + \delta_{n,0}  \sum_{p = 0}^m \frac{5}{2}(2p+1)^2 = \sum_{p = 0}^m \frac{5}{2}(2p+1)^2 \\
	& \quad = \frac{5}{6}(m+1)(2m+1)(2m+3).
	\end{aligned}
	\end{equation}
	Thus the total contribution will be
	\begin{equation}
	(a_E)_{m,n} = \frac{5}{6}(m+1)^2(4m^2+8m+3) = \frac{5}{24}(l+1)(l+2)^2(l+3).
	\end{equation}
	Although $a_E$ doesn't vanish level-by-level, the summation over $n$ will still give zero, consistent with field theory.
	
	\subsubsection{Theory 2: $\cN = 1$ SU(3) $J_n$ theory}
	The theory is connected to the $\cN = 4$ theory discussed above, and the spectrum is provided in \cite{Cesaro:2022mbu}.
	
	We focus on a specific two-parameter U(1)$\times$U(1) solution in 4d dyonically gauged supergravity, which is parametrized by two pseudoscalars $(\chi_1, \chi_2)$. At the special locus $\chi_1 = \chi_2 = 0$, the flavor symmetry is enhanced to SU(3), which is the theory we study here. The contents of 4d $\cN = 1$ multiplets with their irreps under SU(3) are explicitly given in (3.3) and (3.4) of \cite{Cesaro:2022mbu}. For general KK level $(l,n)$, the multiplets are all long. The only exception is $l = n = 0$, where we have MGRAV and MVEC, notice that there will be extra multiplets generated:
	\begin{equation}
	\begin{aligned}
	{\rm LGRAV}[E_0 = \frac{5}{2} + \epsilon] & \rightarrow {\rm MGRAV}[E_0 = \frac{5}{2}] \oplus {\rm LGINO}[E_0 = 3],\\
	{\rm LVEC}[E_0 = \frac{3}{2} + \epsilon] & \rightarrow {\rm MVEC}[E_0 = \frac{3}{2}] \oplus {\rm LSCA}[E_0 = 2].\\
	\end{aligned}
	\end{equation}
	Taking advantage of the coefficients for $\cN = 1$ multiplets given in Table \ref{HeatKernelCoefficientsN=1Multiplets}, we obtain the following coefficients:
	\begin{equation}
	(a_E)_{l,n} = \frac{5}{24}(l+1)(l+2)^2(l+3),\quad c_{l,n} = (b_1)_{l,n} = 0.
	\end{equation}
	The coefficients are identical to the $\cN = 4$ theory level-by-level, providing another supporting example of our conjecture \ref{LogNRGFlowConjecture}.

%%%%%%%%%%%%%%%%%%%%%%%%
\section{Regularizing sums over KK spectra}
\label{app:reg}
%%%%%%%%%%%%%%%%%%%%%%%%


Throughout the main text, we encounter a number of infinite sums that require regularization. In this appendix, we review a couple of methods that can in some cases attach a finite value to a divergent series. We hasten to note that these methods, being essentially based on zeta-function regularization, are neither linear nor stable (see e.g.~\cite{Monin:2016bwf}). As such, we do not claim that they can be used to regularize all infinite sums we encounter in an unambiguous way. But we are inclined to trust these methods whenever they yield results that are compatible with AdS/CFT expectations, as discussed in the main text.\\

The first method is a spectral regularization, which we apply to the sum
\begin{equation}
\label{eq:sum-proto}
\mathcal{S} = \sum_{n\geq0}(n+1)(n+2)(n+3)^2(n+4)(n+5) \, .
\end{equation}
We follow \cite{Gibbons:1984dg}. First, we introduce the following zeta function:
%
\begin{equation}
\label{eq:spectral-zeta}
\zeta_\Delta(z) = 1 + \sum_{n\geq1}D(n)\bigl(n(n+6)\bigr)^{-z} \, ,
\end{equation}
%
where
\begin{equation}
D(n) = \frac{1}{360}(n+1)(n+2)(n+3)^2(n+4)(n+5) \, .
\end{equation}
The function $\zeta_\Delta$ is associated to the scalar Laplacian $\Delta$ on the seven-sphere. Indeed, this differential operator has eigenvalues $n(n+6)$ with $n\geq 0$ and their multiplicities are given by $D(n)$. This spectral zeta function has an integral representation,
%
\begin{equation}
\zeta_\Delta(z) = \frac{1}{\Gamma(z)}\,\int_0^\infty\,t^{z-1}\,\mathrm{Tr}\bigl[e^{-t\Delta}\bigr]\,dt \, ,
\end{equation}
%
and the value of $\zeta_\Delta(0)$ can be obtained from a heat kernel computation as~\cite{gilkey2018invariance}
%
\begin{equation}
\zeta_\Delta(0) = a_{d}(\Delta)\,\text{res}_{z=0}\Gamma(z) \, ,
\end{equation}
%
where $d$ is the dimension of the space on which the scalar Laplacian acts. Crucially, the coefficient $a_d(\Delta)$ vanishes when $d$ is odd~\cite{gilkey2018invariance}, leading to $\zeta_\Delta(0) = 0$ for the seven-sphere. Thus, this method attaches the finite value
\begin{equation}
\mathcal{S} = 0 \, ,
\end{equation} 
to the infinite sum~\eqref{eq:sum-proto}. \\

Another regularization method can be adapted from~\cite{friedman2012special}, and is more general than the spectral zeta-function method. Namely, consider a divergent series of the form
\begin{equation}
\label{eq:sum-proto-gen}
\sum_{n\geq 0} f(n) \, .
\end{equation}
It will be important in what follows that $f$ satisfies the following two properties: (i) $f(n) \neq 0$ for $n \in [0,\infty)$ and, (ii) $f_{\text{top}}(n) = 0$ only for $n=0$. Here the subscript ``top'' indicates the term of highest homogeneity degree in $f$. The way to attach a finite value to~\eqref{eq:sum-proto-gen} is to introduce the zeta function
\begin{equation}
\zeta(s;f) = \sum_{n\geq 0} f(n)^{-s} \, . 
\end{equation}
Then, under the assumptions (i) and (ii) above required for convergence,~\cite{friedman2012special} showed that 
\begin{equation}
\label{eq:FP-zeta-reg}
\zeta(-1;f) = \sum_{L\geq0} c_L(f)\,B_L \, ,
\end{equation}
where $B_L$ is the $L$-th Bernoulli number and $c_L(f)$ is read off from the expansion of
\begin{equation}
\frac{f_a^{[\text{deg}(f)]}}{\text{deg}(f)}\sum_{\ell = 2}^{\text{deg}(f) + 1}\frac{(-1)^{\ell - 1}}{\ell(\ell - 1)}\,C_\ell(f_a) = \sum_{L\geq0} c_L(f)\,a^L \, .
\end{equation}
Here we have defined $f_a(n) = f(n+a)$, 
\begin{equation}
f^{[m]} = \frac{1}{m!} \frac{d^m f(n)}{dn^m}\Big\vert_{n=0} \, , 
\end{equation}
and $C_\ell(f)$ is the coefficient of $y^{1+\text{deg}(f)}$ in
\begin{equation}
\Bigg(\sum_{i=1}^{\text{deg}(f)}\frac{f^{[\text{deg}(f) - i]}}{f^{[\text{deg}(f)]}}\,y^i\Bigg)^\ell \, .
\end{equation}

Let us apply this regularization to the series $\mathcal{S}$ in~\eqref{eq:sum-proto}. We find that the coefficients $c_L$ are given by
%
\begin{equation}
c_L(\mathcal{S}) = \Bigl\{-\frac{738}{7},\,-360,\,-471,\,-\frac{949}{3},\,-120,\,-26,\,-3,\,-\frac{1}{7}\Bigr\} \, ,
\end{equation}
%
for $L=0 \ldots 7$. Remarkably, using this specific linear combination of Bernoulli numbers in~\eqref{eq:FP-zeta-reg} shows that
\begin{equation}
\mathcal{S} = 0 \, ,
\end{equation}
in agreement with the spectral regularization method. We can also use this prescription to attach a finite values to other sums. In Appendix~\ref{App:KK:N010}, we encountered the divergent series 
\begin{equation}
\begin{split}
\mathcal{S}_1 =&\; \frac14\sum_{n\geq 0}(1+n)^3(5 + 2n) \, , \\
\mathcal{S}_2 =&\; -\frac14\sum_{n\geq 0}(1+n)(4+n)(5+2n)^2 \, , \\
\mathcal{S}_3 =&\; \frac14\sum_{n\geq 0}(2+n)^3(1+2n) \, .
\end{split}
\end{equation}
The relevant $c_L$ coefficients are
\begin{equation}
\begin{split}
c_L(\mathcal{S}_1) =&\; \left\{-\frac{1229}{5120},-\frac{5}{4},-\frac{17}{8},-\frac{7}{4},-\frac{11}{16},-\frac{1}{10}\right\}_{L=0\ldots 5} \, , \\[1mm]
c_L(\mathcal{S}_2) =&\; \left\{\frac{125}{16},25,\frac{205}{8},\frac{47}{4},\frac{5}{2},\frac{1}{5}\right\}_{L=0\ldots 5} \, , \\[1mm]
c_L(\mathcal{S}_3) =&\; \left\{-\frac{1267}{5120},-2,-\frac{7}{2},-\frac{5}{2},-\frac{13}{16},-\frac{1}{10}\right\}_{L=0\ldots 5} \, ,
\end{split}
\end{equation}
which lead to the finite values quoted in~\eqref{eq:c-N010-reg}.


%%%%%%%%%%%%%%%%%%%%%%%%%%%%%%%%%%%%%%%%%%%%%%%%%%
% Keep the following \cleardoublepage at the end of this file, 
% otherwise \includeonly includes empty pages.
\cleardoublepage

% vim: tw=70 nocindent expandtab foldmethod=marker foldmarker={{{}{,}{}}}
